# Supplementary material for: Learning Optimal Representations with the Decodable Information Bottleneck
Source: arXiv:2009.12789 source file (2021-07-16)
Supplement: Supplementary file 1 [file proofs_dif.tex]

\subsection{Conditional Information}
\label{sec:proof_dif}

\textbf{decentropy}

It has the following desirable properties
\textbf{propentropy}

\begin{proof}
\begin{description}
\item[Monotonicity] Essentially because the infimum is taken over a larger set.
Let $\family{} \subseteq \pFam{\mathfam{G}}$, $\mathcal{A}_i \defeq \{\E{n_i ,z \sim P_{\rv N_i \times \rv z}}{L(n_i,\pred{}))} \ s.t. \ \pred{} \in \family{} \}$, and $\mathcal{B}_i \defeq \ \{\E{n_i,z \sim P_{\rv N_i \times \rv Y}}{S(n_i,\pred{}))} \ s.t. \ \pred{} \in \pFam{\mathfam{G}} \}$.
The image of a subset under a mapping is the subset of the image, so we have $\mathcal{A}_i \subseteq \mathcal{B}_i$.
By the subset property of infimums $\mathcal{A}_i \subseteq \mathcal{B}_i$ implies $\inf \mathcal{A}_i \geq \inf \mathcal{B}_i$, $\forall \rv N_i \in \rv N $.
As the previous inequality holds for all $\rv N_i$, we have that the inequality also holds for the sum of all terms : $\CHF{X}{Z} = \sum_{\rv N_i \in \rv N} \inf \mathcal{A}_i \geq \sum_{\rv N_i \in \rv N} \inf  \mathcal{B}_i = \op{H_{\mathfam{G}}}{\rv X, \rv Z}$. 
Conclude because $\op{H}{Y}$ is a constant. 
\item[Non negativity] First show it $\DIF{N_i}{Z}$. Because of our assumption on the predictive family we know that there exists a predictor that always predicts using the marginal. Because of the infimum $H_Q[Y|Z]$ can only be smaller than that, so $H[Y]-H_Q[Y|Z]$ has to be greater than 0.
Sum of non negative terms is non negative terms so we have $\DIF{X}{Z}$ because each $\DIF{N_i}{Z}$ are non negative (as just shown).
\item[Independence] 
First we show it for $\DIF{N_i}{Z}$
\begin{align}
\CHF{N_i}{Z} &= \inf_{Q \in Q} \E{n_i ,z \sim P_{\rv N_i \times \rv z}}{- \log q(n_i|z)))}    & \text{definition} \\
&= \inf_{Q \in Q}\E{n_i \sim P_{\rv N_i}}{ \E{z \sim P_{\rv z}}{- \log q(n_i|z)))}}   & \text{independence} \\
&\geq \E{n_i \sim P_{\rv N_i}}{- log \E{z \sim P_{\rv z}}{ q(n_i|z)))}}   & \text{jensen} \\
&= \inf_{Q \in Q} \E{n_i \sim P_{\rv N_i}}{- log q(n_i)))}   & \text{marginalize} \\
&= \op{H}{\rv N_i} &{Strict properness} \\
\end{align}
Where the last line uses the strict properness of the log loss (so the best marginal predict is the underlying marginal) and the fact that we assumed that there is a predictor that always predicts with the true marginal in $\mathfam{Q}$.
We thus have $\op{H}{\rv N_i} - \CHF{N_i}{Z} \leq 0 $ but we know that positive (proved above) so $\DIF{N_i}{Z}=0$.
Let's tackle $\DIF{X}{Z}$, we know that if $\rv X \perp \rv Z$ then $\MI{X}{Z}=0$. As MI is invariant to bijections and $\rv N_i$ are independent we have $0=\MI{X}{Z}=\MI{\{\rv N_i\}_i}{Z}=\sum_{\rv N_i}=\MI{N_i}{Z}$ from which we conclude that each $\rv N_i$ is independence of $\rv Z$. 
We can thus apply our previous proof on each component $\DIF{X}{Z}=\sum_{\rv N_i} \DIF{N_i}{Z}=0$.
\end{description}
\end{proof}

Let's now prove that we generalize MI and $\mathcal{V}$ information.

\begin{lemma}[Decomposition and Recoverability of Conditional Entropy]\label{lem:weak}
Let $\rv N = ( \rv N_i )_i$ be a random vector with component $\rv N_i$ then $\sum_{\rv N_i \in \rv N } \inf_{U \in \mathfam{U}} \E{n_i,z \sim P_{\rv N_i \times \rv z}}{S(n_i,U_{\hrv N_i \cond z}))} = \op{H}{\rv X \cond \rv Z }$ $\forall \rv Z$ if and only if $\rv N$ is a $\mathcal{Y}$ decomposition of $\rv X$.
\end{lemma}

\begin{proof}
\begin{description}
\item[Take value in $\mathcal{Y}$] Suppose $\exists i \ s.t. \ \rv N_i$ does not satisfy the $\mathcal{Y}$-requirement. Then there exists $n_i \not\in \mathcal{Y}$, which happens with non zero probability. As a result, $S(n_i,U_{\hrv N_i \cond z}))=- \log(U_{\hrv N_i \cond z}(n_i \cond z))$ is not well defined (because the codomain of $U_{\hrv N_i \cond z}$ is wrong) . The expectation over $\rv N_i$ is thus also not well defined (as $U$ t.v.i in $\mathcal{P}(\mathcal{Y})$ ).
\item[Bijection and Independence] 
First let us show that if $\rv N$ is a $\mathcal{Y}$ decomposition of $\rv X$ , then $\sum_{\rv N_i \in \rv N } \inf_{U \in \mathfam{U}} \E{n_i,z \sim P_{\rv N_i \times \rv z}}{S(n_i,U_{\hrv N_i \cond z}))} = \op{H}{\rv X \cond \rv Z }$:
\begin{align*}
\op{\Tilde{H}_{\mathfam{U}}}{\rv X \cond \rv Z} &= \sum_{\rv N_i \in \rv N } \inf_{U \in \mathfam{U}} \E{n_i,z \sim P_{\rv N_i \times \rv z}}{S(n_i,U_{\hrv N_i \cond z}))} \\
&= \sum_{\rv N_i \in \rv N } \E{n_i,z \sim P_{\rv N_i \times \rv z}}{S(n_i,P_{\hrv N_i \cond  z}(n_i \cond z)} & \text{Strictly Proper} \\
&= \sum_{\rv N_i \in \rv N } \op{H}{\rv N_i \cond \rv Z} & \text{Definition} \\
&= \op{H}{(\rv N_i)_i \cond \rv Z} & \text{Independence} \\
&= \op{H}{f((\rv N_i)_i) \cond \rv Z} & \text{bijection req.} \\
&= \op{H}{\rv X \cond \rv Z} 
\end{align*}
Where the second line uses the strict properness of the log loss and the fact that $P_{N_i \cond \rv z} \in \PYZ = \universal{}$. 
Where the last line comes from the assumption that there exists a bijection $f$ s.t. $\rv X = f(\rv N)$.
This proves the first direction. 

For the other direction , suppose that $\sum_{\rv N_i \in \rv N } \inf_{U \in \mathfam{U}} \E{n_i,z \sim P_{\rv N_i \times \rv z}}{S(n_i,U_{\hrv N_i \cond z}))} = \op{H}{\rv X \cond \rv Z }$ $\forall \rv Z$.
Using the strict properness of the log loss (as before) we get that $\sum_{\rv N_i \in \rv N } \op{H}{\rv N_i \cond \rv Z} = \op{H}{\rv X \cond \rv Z}, \ \forall Z$.

Set $\rv Z = \rv X$ then $\sum_{\rv N_i \in \rv N } \op{H}{\rv N_i \cond \rv X} = \op{H}{\rv X \cond \rv X} = 0$. 
As conditional entropy is non-negative (discrete case), then we must have $\op{H}{\rv N_i \cond \rv X}=0, \ \forall i$. From which we conclude that $\forall i$ there exists $f_i$ s.t. $\rv N_i = f_i(\rv X)$.
Similarly set $\rv Z = \rv N$ then $\op{H}{\rv N_i \cond \rv N}=0, \ \forall N_i \in \rv N$ so $\op{H}{\rv X \cond \rv N } = \sum_{\rv N_i \in \rv N } \op{H}{\rv N_i \cond \rv N} = 0$ from which we conclude that there is a function $f^{-1}$ s.t. $\rv X = f^{-1}(\rv N)$. 
Putting it with the previous equation we have $\rv X = f^{-1}(\rv N) = f^{-1}((\rv N_i)_i) =  f^{-1}(( f_i(\rv X) )_i)$ from which we conclude that $f(\cdot)=(f_i(\cdot))_i$ is a bijection.

Finally, suppose $\rv Z$ is independent of $\rv X$. As there exists a bijection between $\rv N$ and $\rv X$ we also have that $\rv Z \perp \rv N$ so
\begin{align*}
\op{H}{\rv X } 
&= \op{H}{\rv X \cond \rv Z} & \rv Z \perp \rv X \\
&= \sum_{\rv N_i \in \rv N } \op{H}{\rv N_i \cond \rv Z} \\
&= \sum_{\rv N_i  } \op{H}{\rv N_i} & \rv Z \perp \rv N \\
&\geq \op{H}{(\rv N_i)_i }  \\
&= \op{H}{f((\rv N_i)_i)} & \text{\cref{cor:bij}} \\
&= \op{H}{\rv X } 
\end{align*}
Obviously $\op{H}{\rv X } = \op{H}{\rv X} $ so the inequality has to be an equality $\sum_{\rv N_i } \op{H}{\rv N_i} = \op{H}{(\rv N_i)_i }$. I.e. $\rv N_i \perp \rv N_j, \forall i \neq j$, which concludes the proof.
\end{description}
\end{proof}

\textbf{specialcase}

\begin{proof}
\begin{description}
\item[$\mathcal{V}$-information] The simplest $\mathcal{Y}$ decomposition of $\rv Y$ is $\rv N= \{\rv Y\}$. In this case there is only one element in the sum, and the definition the decodable information becomes the same as the $\mathcal{V}$-information. Any $\rv N= \{f(\rv Y)\}$ where $f$ is a bijection, would also be a valid $\mathcal{Y}$ decomposition, but that would not change the decodable entropy \ydnote{write in math all of that} because the predictive family is invariant to bijections on $\mathcal{Y}$.
We now have to show that with the assumptions made $\op{H}{\rv Y} = \op{H_\mathcal{V}}{\rv Y | \varnothing}$ \ydnote{shoudl rewrite their definition and optional ignorance !} . $\op{H_\mathcal{V}}{\rv Y | \varnothing}$ does not take into account the input, in which case \ydnote{write that formally} the best predictor is the underlying marginal (because of strict properness). Because of our assumption on the predictive family we can always predict using the underlying marginal so $\op{H}{\rv Y} = \op{H_\mathcal{V}}{\rv Y | \varnothing}$.
\item[Mutual Information] Given the form of the decodable entropy (link) equation, we can apply \cref{lem:weak}, and conclude that $\mathfam{U}$ decodable entropy recovers coditional entropy if and only if $(\rv N_i)_i$ is a $\mathcal{Y}$ decomposition of $\mathcal{X}$.
We thus have $\op{H}{X|Z}=\op{H_{\mathfam{U}}}{X|Z}$.
As $\{ \rv N_i\}$ is a decomposition of $\rv X$ we also have $\op{H}{\rv X}=\sum_{\rv N_i} \op{H}{\rv N_i}$.
Putting all together $\DI{\mathcal{U}}{X}{Z} = (\sum_{\rv N_i} \op{H}{\rv N_i}) - \op{H_{\mathfam{U}}}{X}{Z} = \op{H}{\rv X} - \op{H}{X|Z} = \MI{X}{Z}$.
\end{description}
\end{proof}
