# Supplementary material for: Learning Optimal Representations with the Decodable Information Bottleneck
Source: arXiv:2009.12789 source file (2021-07-16)
Supplement: Supplementary file 2 [file randlab.tex]

\subsection{The Importance of Base $|\mathcal{Y}|$ Expansion Labeling}
\label{sec:appx_randlab}

\yann{Unreferenced}

\david{Rewrite if algorithm stays here}
\Cref{theo:opt_qmin} states that representations that maximize $\CHF{X}{Z}$ are optimal.
But the same holds [cite lemma] for representations that minimize the predictability of any random label.
In \cref{sec:theory_opt_rep} we argued that we are effectively minimizing the predictability of random labels [cite lemma] but propose a way to use only a specific set of possible labels of cardinality $\log_{|\mathcal{Y}|}(\mathcal{X})$ instead of all $|\mathcal{Y}|^{|\mathcal{X}|}$ possible random labels.
One interesting practical question is whether using these specific possible labels is better than randomly selecting the same number of possible labels from the entire set.
Indeed, although the former are optimal then latter might also be good  as [talk about the fact that typical sets have high entropy and low correlation => likely will cover].

\input{figures/algorithms/baseb}

\subsection{The Importance of Base $|\mathcal{Y}|$ Expansion Labeling}
\label{sec:appx_randlab}

\yann{Unreferenced}

\david{Rewrite if algorithm stays here}
\Cref{theo:opt_qmin} states that representations that maximize $\CHF{X}{Z}$ are optimal.
But the same holds [cite lemma] for representations that minimize the predictability of any random label.
In \cref{sec:theory_opt_rep} we argued that we are effectively minimizing the predictability of random labels [cite lemma] but propose a way to use only a specific set of possible labels of cardinality $\log_{|\mathcal{Y}|}(\mathcal{X})$ instead of all $|\mathcal{Y}|^{|\mathcal{X}|}$ possible random labels.
One interesting practical question is whether using these specific possible labels is better than randomly selecting the same number of possible labels from the entire set.
Indeed, although the former are optimal then latter might also be good  as [talk about the fact that typical sets have high entropy and low correlation => likely will cover].

\input{figures/algorithms/baseb}

\Cref{fig:randlab} compares the effect of using [5,15,25,50,100] random labels instead of base expansions on Alice's log likelihood.
All other hyperparameters are identical to the ones used to generate \cref{fig:qmin_joint}.
For comparison, we also trained a DIB model which minimizes the base expansion for different indexing of $\mathcal{X}$.
Indeed, increasing the number of random labels might help as we do not have access to a global optimizer and each head will find different predictors due to their different initialization.
We see that ...

As discussed in \cref{sec:practical_optim}, the DIB formulation (like the IB formulation) gives rise to a trade-off between removing information about the input and preserving information about the label.
Such trade-off comes from Lagrangian relaxation.
To illustrate this, let's look at the IB objecive and its solution : minimal sufficient representations.
Due to the sufficient constraint we have $\op{H}{\rv Y \cond \rv Z }$ is a constant, meaning that maximizing $\op{H}{\rv X \cond \rv Z }$ cannot remove information about $\rv Y$ from $\rv Z$:

\begin{align*}
\smin{} &\defeq \arg \max_{Z \in \suff{}} \op{H}{\rv X \cond \rv Z } \\
&= \arg \max_{Z \in \suff{}} \op{H}{\rv X , \rv Y \cond \rv Z } & \rv Y - \rv X - \rv Z\\
&= \arg \max_{Z \in \suff{}} \op{H}{\rv X  \cond \rv Z , \rv Y}  + \op{H}{\rv Y \cond \rv Z }  & \text{Chain Rule} \\
&= \arg \max_{Z \in \suff{}} \op{H}{\rv X  \cond \rv Z , \rv Y}   + (Const)  & \text{Sufficiency} \\
&= \arg \max_{Z \in \suff{}} \op{H}{\rv X  \cond \rv Z , \rv Y}  
\end{align*}

We see that minimal representations can  be recovered by minimizing $\op{H}{\rv X  \cond \rv Z , \rv Y}$ instead of $\op{H}{\rv X  \cond \rv Z}$.
This can also be seen in the IB loss by incrementing $\beta$ by 1:

\begin{align*}
\mathcal{L}_{IB}^{\beta + 1}&= 
\op{I}{\rv X ; \rv Z} - (\beta+1) \op{I}{\rv y ; \rv Z} \\
&= 
\op{I}{\rv X, \rv Y ; \rv Z } - \op{I}{\rv y ; \rv Z} - \beta \op{I}{\rv y ; \rv Z} \\
&= 
\op{I}{\rv X ; \rv Z \cond \rv Y} + \op{I}{\rv y ; \rv Z} - \op{I}{\rv y ; \rv Z} - \beta \op{I}{\rv y ; \rv Z} \\ 
&= 
\op{I}{\rv X ; \rv Z \cond \rv Y}  - \beta \op{I}{\rv y ; \rv Z} \\ 
&= 
\mathcal{L}_{CIB}^{\beta }
\end{align*}

In theory, $\mathcal{L}_{CIB}^{\beta }$ is thus not very helpful as it is equivalent to $\mathcal{L}_{IB}$ with a different $\beta$.
In practice though, this might give rise to very different solutions as the estimation procedure can be different.
In the variational estimation case, this has been discussed in \cite{CIB}.

In our case we maximize  $\CHF{X}{Z}$ while minimizing $\CHF{Y}{Z}$ to make sure that no decodable information about $\rv Y$ is removed.
As we use an approximation procedures for optimization (no global optima), it is very probable that we end up removing a lot of information about $\rv Y$ when trying to remove information about $\rv X$.
To avoid this issue, we would also like to optimize $\op{H_{\V}}{\rv X   \cond  \rv Z}$ without changing $\op{H_{\V}}{\rv Y   \cond \rv Z}$.
We see two ways of doing it :

\begin{itemize}
\item $\Qsmin{} = \arg \max_{\rv z \in \Qsuff{}}\CHF{X}{Z} - \CHF{Y}{Z}$, which we will refer to as $\Delta$ DIB.
This might seem useless as it still requires estimating $\CHF{X}{Z}$. 
But (in some cases) we can actually directly estimate $\CHF{X}{Z} - \CHF{Y}{Z}$ without computing $\CHF{X}{Z}$.
Indeed, $\CHF{X}{Z} \defeq \sum_{\rv N_i \in \rv N} \CHF{N_i}{Z} $ so if we can set one of $\rv N_i$ to be equal to  $\rv Y$ then $\CHF{X}{Z} - \CHF{Y}{Z} = \sum_{\rv N_i \neq \rv Y} \CHF{N_i}{Z}$.
Practically this means that we need one less head and only need to remove predictability of indices in a given class (i.e. start indexing from 0 for every class).
The only problem with this, is that it is only exact if each $\rv N_i$ are independent (which is the case for balanced datasets).
\item $\Qsmin{} = \arg \max_{\rv z \in \Qsuff{}} \op{H_{\V}}{\rv X   \cond  \rv Z, \rv Y}$, which we will refer to as Conditional DIB.
This requires defining $\op{H_{\V}}{\rv X   \cond  \rv Z, \rv Y}$, which is not straightforward as $\V$ has $\mathcal{Z}$ as domain, not $\mathcal{Z}\times\mathcal{Y}$.
This can nevertheless be done exactly \ydnote{by exactly I mean that I keep the recoverability of $\op{H}{\rv X   \cond  \rv Z, \rv Y}$ } :
\begin{align*}
\op{H_{\V}}{\rv X   \cond  \rv Z, \rv Y} &\defeq \E{y \in P_{\rv Y}}{\op{H_{\V}}{\rv X   \cond  \rv Z, y}} \\
&= \E{y \in P_{\rv Y}}{\sum_{\rv N_i} \inf_{Q \in \V} \sum_n \sum_x \sum_z p(x,n \cond y) p(z \cond x, n, y) \log q(n \cond z, y))} \\
&= \E{y \in P_{\rv Y}}{\sum_{\rv N_i} \inf_{Q \in \V} \sum_n \sum_x \sum_z p(x,n \cond y) p(z \cond x) \log q(n \cond z))}
\end{align*}
The key is to realize that $q(n \cond z, y)=q(n \cond z)$ as the infimum is taken inside the expectation over $\rv Y$.
Practically speaking it means that for a given possible labeling $\rv N_i$ we do not need to use a single predictor but can use a different predictor for each class.
This is always possible, but suffers from the fact that it needs a number of predictors that is linear in $|\mathcal{Y}|$.
\end{itemize}

\input{figures/cdib/cdib}

We hypothesize that the Conditional and the $\Delta$ DIB objectives \ydnote{I will also look at the approximated CDIB by concatenating Y to Z. But probably won't put it in the paper, as it's hard to motivate theoretically (although practically will probably work well).} will be much more robust to varying $\beta$ than DIB and might even remove the need of hyperparamer tuning $\beta$ altogether. 
We compare both methods, and the non conditional version in \cref{fig:cdib} and see that ....

\Cref{fig:randlab} compares the effect of using [5,15,25,50,100] random labels instead of base expansions on Alice's log likelihood.
All other hyperparameters are identical to the ones used to generate \cref{fig:qmin_joint}.
For comparison, we also trained a DIB model which minimizes the base expansion for different indexing of $\mathcal{X}$.
Indeed, increasing the number of random labels might help as we do not have access to a global optimizer and each head will find different predictors due to their different initialization.
We see that ...

As discussed in \cref{sec:practical_optim}, the DIB formulation (like the IB formulation) gives rise to a trade-off between removing information about the input and preserving information about the label.
Such trade-off comes from Lagrangian relaxation.
To illustrate this, let's look at the IB objecive and its solution : minimal sufficient representations.
Due to the sufficient constraint we have $\op{H}{\rv Y \cond \rv Z }$ is a constant, meaning that maximizing $\op{H}{\rv X \cond \rv Z }$ cannot remove information about $\rv Y$ from $\rv Z$:

\begin{align*}
\smin{} &\defeq \arg \max_{Z \in \suff{}} \op{H}{\rv X \cond \rv Z } \\
&= \arg \max_{Z \in \suff{}} \op{H}{\rv X , \rv Y \cond \rv Z } & \rv Y - \rv X - \rv Z\\
&= \arg \max_{Z \in \suff{}} \op{H}{\rv X  \cond \rv Z , \rv Y}  + \op{H}{\rv Y \cond \rv Z }  & \text{Chain Rule} \\
&= \arg \max_{Z \in \suff{}} \op{H}{\rv X  \cond \rv Z , \rv Y}   + (Const)  & \text{Sufficiency} \\
&= \arg \max_{Z \in \suff{}} \op{H}{\rv X  \cond \rv Z , \rv Y}  
\end{align*}

We see that minimal representations can  be recovered by minimizing $\op{H}{\rv X  \cond \rv Z , \rv Y}$ instead of $\op{H}{\rv X  \cond \rv Z}$.
This can also be seen in the IB loss by incrementing $\beta$ by 1:

\begin{align*}
\mathcal{L}_{IB}^{\beta + 1}&= 
\op{I}{\rv X ; \rv Z} - (\beta+1) \op{I}{\rv y ; \rv Z} \\
&= 
\op{I}{\rv X, \rv Y ; \rv Z } - \op{I}{\rv y ; \rv Z} - \beta \op{I}{\rv y ; \rv Z} \\
&= 
\op{I}{\rv X ; \rv Z \cond \rv Y} + \op{I}{\rv y ; \rv Z} - \op{I}{\rv y ; \rv Z} - \beta \op{I}{\rv y ; \rv Z} \\ 
&= 
\op{I}{\rv X ; \rv Z \cond \rv Y}  - \beta \op{I}{\rv y ; \rv Z} \\ 
&= 
\mathcal{L}_{CIB}^{\beta }
\end{align*}

In theory, $\mathcal{L}_{CIB}^{\beta }$ is thus not very helpful as it is equivalent to $\mathcal{L}_{IB}$ with a different $\beta$.
In practice though, this might give rise to very different solutions as the estimation procedure can be different.
In the variational estimation case, this has been discussed in \cite{CIB}.

In our case we maximize  $\CHF{X}{Z}$ while minimizing $\CHF{Y}{Z}$ to make sure that no decodable information about $\rv Y$ is removed.
As we use an approximation procedures for optimization (no global optima), it is very probable that we end up removing a lot of information about $\rv Y$ when trying to remove information about $\rv X$.
To avoid this issue, we would also like to optimize $\op{H_{\V}}{\rv X   \cond  \rv Z}$ without changing $\op{H_{\V}}{\rv Y   \cond \rv Z}$.
We see two ways of doing it :

\begin{itemize}
\item $\Qsmin{} = \arg \max_{\rv z \in \Qsuff{}}\CHF{X}{Z} - \CHF{Y}{Z}$, which we will refer to as $\Delta$ DIB.
This might seem useless as it still requires estimating $\CHF{X}{Z}$. 
But (in some cases) we can actually directly estimate $\CHF{X}{Z} - \CHF{Y}{Z}$ without computing $\CHF{X}{Z}$.
Indeed, $\CHF{X}{Z} \defeq \sum_{\rv N_i \in \rv N} \CHF{N_i}{Z} $ so if we can set one of $\rv N_i$ to be equal to  $\rv Y$ then $\CHF{X}{Z} - \CHF{Y}{Z} = \sum_{\rv N_i \neq \rv Y} \CHF{N_i}{Z}$.
Practically this means that we need one less head and only need to remove predictability of indices in a given class (i.e. start indexing from 0 for every class).
The only problem with this, is that it is only exact if each $\rv N_i$ are independent (which is the case for balanced datasets).
\item $\Qsmin{} = \arg \max_{\rv z \in \Qsuff{}} \op{H_{\V}}{\rv X   \cond  \rv Z, \rv Y}$, which we will refer to as Conditional DIB.
This requires defining $\op{H_{\V}}{\rv X   \cond  \rv Z, \rv Y}$, which is not straightforward as $\V$ has $\mathcal{Z}$ as domain, not $\mathcal{Z}\times\mathcal{Y}$.
This can nevertheless be done exactly \ydnote{by exactly I mean that I keep the recoverability of $\op{H}{\rv X   \cond  \rv Z, \rv Y}$ } :
\begin{align*}
\op{H_{\V}}{\rv X   \cond  \rv Z, \rv Y} &\defeq \E{y \in P_{\rv Y}}{\op{H_{\V}}{\rv X   \cond  \rv Z, y}} \\
&= \E{y \in P_{\rv Y}}{\sum_{\rv N_i} \inf_{Q \in \V} \sum_n \sum_x \sum_z p(x,n \cond y) p(z \cond x, n, y) \log q(n \cond z, y))} \\
&= \E{y \in P_{\rv Y}}{\sum_{\rv N_i} \inf_{Q \in \V} \sum_n \sum_x \sum_z p(x,n \cond y) p(z \cond x) \log q(n \cond z))}
\end{align*}
The key is to realize that $q(n \cond z, y)=q(n \cond z)$ as the infimum is taken inside the expectation over $\rv Y$.
Practically speaking it means that for a given possible labeling $\rv N_i$ we do not need to use a single predictor but can use a different predictor for each class.
This is always possible, but suffers from the fact that it needs a number of predictors that is linear in $|\mathcal{Y}|$.
\end{itemize}

\input{figures/cdib/cdib}

We hypothesize that the Conditional and the $\Delta$ DIB objectives \ydnote{I will also look at the approximated CDIB by concatenating Y to Z. But probably won't put it in the paper, as it's hard to motivate theoretically (although practically will probably work well).} will be much more robust to varying $\beta$ than DIB and might even remove the need of hyperparamer tuning $\beta$ altogether. 
We compare both methods, and the non conditional version in \cref{fig:cdib} and see that ....
