# Supplementary material for: Learning Optimal Representations with the Decodable Information Bottleneck
Source: arXiv:2009.12789 source file (2021-07-16)
Supplement: Supplementary file 3 [file algorithm.tex]

\label{appx:algorithm}
