# Supplementary material for: Learning Optimal Representations with the Decodable Information Bottleneck
Source: arXiv:2009.12789 source file (2021-07-16)
Supplement: Supplementary file 4 [file proof_min_old.tex]

\subsection{$\V$-Minimality}
\ydnote{Keep for Arxive?}

In this section we will formalize all the necessary tools to understand the two following subsections about $\V$-minimality.
We will formalize the necessary definitions and then prove lemmas that will be useful.

\subsubsection{Definitions}
\label{appx:formal_definitions}

First, let us review the notion of $\rv Y$ decomposition of $\rv X$.

\begin{restatable}{definition}{decomposition}\label{def:decomposition}
Let $\mathcal{X}_y \defeq \{ x \in \mathcal{X} \ | \ t(x)=y \}$ be the examples labeled with $y$, and
$\mathcal{T}_y \defeq \{ t' \ | \ t' : \mathcal{X}_y \to \mathcal{Y} \}$ be all possible labeling of $\mathcal{X}_y$. 
The $y$ decomposition of $\rv X$ is 
\[
\mathrm{Dec}(\rv X, y) \defeq \{ \rv N \ | \ \exists t' \in \mathcal{T}_y \ s.t. \ P_{\rv N|y} = t'_{*}(P_{\rv X|y}) \}
\]
where $t'_{*}(P_{\rv X|y})$ is the push forward of $P_{\rv X|y}$ by $t'$.
\end{restatable}


In the main text we only defined $\V$-minimal $\V$-sufficient, but we can also define a similar notion with respect to different functional families.

\begin{restatable}{definition}{GminVsuf}\label{def:GminVsuf}
A representation $\rv Z$ is $\mathcal{G}$-minimal and  $\V$-sufficient if $\rv Z \in  \arg \min_{\rv Z \in \Qsuff{}} \op{I_\mathcal{G}}{\rv Z \rightarrow \decxY{} }$.
\end{restatable}

Now let us formalize the notion of empirical risk minimizer (ERM).

\begin{restatable}{definition}{ERM}\label{def:ERM}
Let $\sampleD{}$ be a sampled dataset.
A predictor $\hat{f}^* \in \V$ is an empirical risk minimizer (ERM) using $\rv Z$ t.v.i. $\mathcal{Z}$  for $\mathcal{D}$ if 
\[
\eqCH{\hat{f}^*}{Y}{Z}{D} = \eCHF{Y}{Z}{D}
\]
We denote the set of ERMs as $\hat{\V}^*(\mathcal{D}, \rv Z)$.
\end{restatable}


\subsubsection{Lemmas}
\label{appx:proof_lemmas}


In this subsection we will prove a collection of lemmas that are useful for the two following sections that prove \cref{theo:opt_qmin} and \cref{prop:Vminsuff}.
Note that these lemmas use the three additional assumptions discussed in the second part of \cref{sec:appx_assumptions}.


For all $\V$-sufficient representations the best achievable test loss is always zero.




If the representation is $\V$-sufficient then it can be partitioned by $\mathcal{Y}$.
I.e. the supports of  each $\rv Z_y$ are non-overlapping.

\begin{restatable}{lemma}{VsuffSupp}\label{lemma:VsuffSupp}
$\rv Z \in \Qsuff{} \implies$ $\mathrm{supp}(P_{\rv Z | y}) \cap \mathrm{supp}(P_{\rv Z | y'}) = \varnothing$, $\forall y\neq y', \ y,y' \in \mathcal{Y}$.
\end{restatable}
\begin{proof}
Let us prove it by contrapositive. 
Namely, we will show $\mathrm{supp}(P_{\rv Z | y}) \cap \mathrm{supp}(P_{\rv Z | y'}) \neq \varnothing \implies \rv Z \not \in \Qsuff{}$.
$\mathrm{supp}(P_{\rv Z | y}) \cap \mathrm{supp}(P_{\rv Z | y'}) \neq \varnothing$ implies that $\exists y \neq y' \in \mathcal{Y}, \exists z \in \mathcal{Z}$ s.t. $P_{\rv Z | \rv Y}(z|y')  \neq 0$ and $P_{\rv Z | \rv Y}(z|y) \neq 0$.
Using Bayes rule, that means $P_{\rv Y | \rv Z}(y'|z)   \neq 0$ and $P_{\rv Y | \rv Z}(y|z)  \neq 0$ so $\nexists y \in \mathcal{Y}$ s.t. $P_{\rv Y | \rv Z}(y'|z) =  1$.
Due to the finite sample space assumption, this implies $0 < \op{H}{\rv Y \cond \rv Z}  = \CHU{Y}{Z}  \leq \CHF{Y}{Z} $. 
From \cref{lemma:perfecttest} we conclude that $\rv Z \not \in \Qsuff{}$ as desired.
\end{proof}

If the representation is $\V$-sufficient then there always exists at least one predictor that is optimal for training and for testing.

\begin{restatable}{lemma}{existperfect}\label{lemma:existperfect}
$\forall \family{}$, $\forall \rv Z \in \Qsuff{}$ there exists $ f \in \family{}$ s.t. $\forall \mathcal{D} \sim P_{\rv Z \times \rv Y}^N $, $\qCHF{Y}{z}=\CHF{Y}{z}=\eqCHF{Y}{z}{D}=\eCHF{Y}{z}{D}=0$
\end{restatable}


\begin{proof}
From \cref{lemma:perfecttest} we know that $\forall Z \in \Qsuff{}$ we have $\CHF{Y}{Z}=0$.
Select any $\rv Z \in \Qsuff{}$ and let $f \in \family{}$ be one of the optimal predictor $\qCHF{Y}{Z}=0$. 
As $\qCHF{Y}{Z}$ is an expectation of a non-negative discrete r.v., it is equal to zero if and only if  $\forall z \in \mathrm{supp}(\rv Z), \ \forall y \in \mathrm{supp}(\rv Y)$  we have $\log f[z](y)=0$.
$\eqCHF{Y}{Z}{D}$ is also a weighted average (discrete expectation) of $\log f[z](y)=0$ over a subset of the previous support $\hat{z} \in \mathrm{supp}(\hrv Z) \subseteqq \mathrm{supp}(\rv Z), \ \forall \hat{y} \in \mathrm{supp}(\hrv Y) \subseteqq \mathrm{supp}(\rv Y)$ so we conclude that $\eqCHF{Y}{Z}{D}=0$.
We thus found a classifier that reaches zero loss, so $\eCHF{Y}{Z}{D}=0$ (infimum and non negativity of log loss).
Putting all together, $\forall Z \in \Qsuff{}$ we have $\CHF{Y}{Z}=\eCHF{Y}{Z}{D}=\qCHF{Y}{Z}=\eqCHF{Y}{Z}{D}=0$ as desired.
\end{proof}



A representation is $\V$-minimal $\V$-sufficient if and only if it has no $\V$-information with any of the terms in the $\rv Y$ decomposition of $\rv X$.

\begin{restatable}{lemma}{zeroVminimal}\label{lemma:zeroVminimal}
$\forall \rv Z \in \Qsmin{} \iff \rv Z \in \Qsuff{}$ and $\forall y \in \mathcal{Y}, \forall \rv N \in \decxy{}$ we have $\DIF{N}{Z_y}=0$. 
\end{restatable}

\begin{proof} $ $ \\
($\impliedby$) Due to the non negativity of $\V$-information, we have $\forall \rv Z' \in \Qsuff{}$,  $0=\DIF{N}{Z_y} \leq \DIF{N}{Z'_y} $ so $\rv Z$ reaches the minimal achievable value in each term and thus also on their expectation $\DIFxzCy{}=0$. We thus conclude that $\rv Z \in \Qsmin{} \defeq \arg \min_{\rv Z \in \Qsuff{}} \DIFxzCy{}$.

($\implies$) 
Let us show that there is at least one $\rv Z \in \Qsmin{}$ s.t. $\forall y \in \mathcal{Y}, \forall \rv N \in \decxy{}, \ \DIF{N}{Z_y}=0 $, from which we will conclude that they all have to in order to minimize $\DIFxzCy{}$.
Note that $P_{\rv Z_y^* \cond \rv X_y}(z_y|x_y) = \frac{1}{|\preimage{f}{t(x_y)}|} = \frac{1}{|\preimage{f}{y}|} = P_{\rv Z_y^*}(z_y)$, where the last equality comes from the fact that $z_y$ is associated with a single label $y$.
An other way of saying it, is that $\rv X_y - y - \rv Z_y$ forms a Markov Chain, but $y$ is a constant.
We thus conclude $\rv Z_y^* \perp \rv X_y$, and because $\rv N = t'( \rv X_y)$ we also have $\rv Z_y^* \perp \rv N$, $\forall \rv N \in \decxy{}$. What we said holds $\forall y \in \mathcal{Y}$. And due to the the independence property of $\V$-information, we have $\DIF{N}{Z_y}=0$ as desired.
As we found one $\rv Z^* \in \Qsmin{}$ s.t. this is true, it must be for all $\rv Z \in \Qsmin{}$.
Indeed, due to the  positivity property it is the only way of reaching the minimal $\DIFxzCy{}=0$.
\end{proof}

Universal sufficient representation corresponds to the subset of sufficient representations that t.v.i. in the domain of predictors in $\universal{}$.

\begin{restatable}[Recoverability of sufficiency]{lemma}{recsuff}\label{prop:recsuff}
 Let $\universal{} = \PYZ{}$ be the universal family, then  $\Usuff{} = \suff{} \cap \mathcal{Z}$
\end{restatable}
\proof{
Let us denote $\Omega = \cup \mathcal{Z}$ as the set of all possible finite sample spaces.
We know that,  $\DI{\universal{}}{Y}{Z} = \MI{Y}{Z}$ so $\arg \min_{\rv Z \in \mathcal{Z}} \DI{\universal{}}{Y}{Z} = \arg \min_{\rv Z \in \mathcal{Z}} \MI{Y}{Z}$. Let us suppose that $\suff{} \cap \mathcal{Z}$ is non empty we have $\suff{} \cap \mathcal{Z} = ( \arg  \min_{\rv Z \in \Omega} \MI{Y}{Z} ) \cap \mathcal{Z}  =  \arg \min_{\rv Z \in \mathcal{Z}} \MI{Y}{Z} = \Usuff{}$ as desired.
To show that $\suff{} \cap \mathcal{Z}$ is indeed non empty, notice that one can always learn the sufficient representation $ \rv Z =\rv Y $  due to the assumption $|\mathcal{Y}| \leq |\mathcal{Z}|$ (when $|\mathcal{Y}| < |\mathcal{Z}|$, restrict the support to $\mathcal{Y}$) and the determinism of $\rv Y$.
}

Let us characterize the set of minimal sufficient representations in terms of independence.

\begin{restatable}[Characterization of Minimal Sufficient Representations]{lemma}{charminsuff}\label{prop:charminsuff}
Suppose $\rv Y $ is a deterministic function of $\rv Y = g(\rv X)$ then the set of minimal sufficient representations correspond to  $\smin{} = \{ \rv Z \in \suff{} | \ \ \rv Z \perp \rv X | \rv Y  \ \}$
\end{restatable}
\proof{
\begin{align*}
\smin{} &\defeq \arg \min_{Z \in \suff{}} \MI{X}{Z} \\
&= \arg \min_{Z \in \suff{}} \MI{X,g(\rv X)}{Z} & \text{Inv. bijections} \\
&= \arg \min_{Z \in \suff{}} \MI{X,\rv Y}{Z} & \text{Det. Labels} \\
&= \arg \min_{Z \in \suff{}} \op{I}{\rv X; \rv Z | \rv Y} + \MI{Z}{Y}   & \text{Chain Rule} \\
&= \arg \min_{Z \in \suff{}} \op{I}{\rv X; \rv Z | \rv Y}   & \text{Sufficiency} 
\end{align*}
Where the second line used the fact that $f(\rv X) = (\rv X, g(\rv X))$ is a bijection.
Notice that $\op{I}{\rv Y; \rv Z | \rv Y} \geq 0$ and we know that it can reach zero, for example with $\rv Z = \rv Y$ (which is sufficient).
So $\smin{} = \{ \rv Z \in \suff{} | \op{I}{\rv Y; \rv Z | \rv Y} = 0\} = \{ \rv Z \in \suff{} | \ \  \rv Z \perp \rv X | \rv Y  \ \}$ which concludes the proof.
}

Similarly, let us characterize the set of $\universal{}$-minimal $\universal{}$-sufficient representations in terms of independence.

\begin{restatable}[Characterization of $\universal{}$-Minimal $\universal{}$-Sufficient Representations]{lemma}{charUminUsuff}\label{prop:charUminUsuff}
Suppose $\rv Y $ is a deterministic function of $\rv Y = g(\rv X)$ then the set of minimal sufficient representations correspond to  $\Usmin{} = \{ \rv Z \in \Usuff{} | \ \forall y \in \mathcal{Y},  \forall \rv N_i \in \mathrm{Dec}(\rv X, y), \ \rv Z \perp \rv N_i  \  \ \}$
\end{restatable}
\begin{proof}
Because of \cref{lemma:zeroVminimal} we have $\forall y \in \mathcal{Y}, \forall \rv N \in \decxy{}$ we have $\DIF{N}{Z_y}=0$.
As $\universal{}$-information recovers MI that means $\rv N \perp \rv Z_y$. So $\Usmin{} = \{ \rv Z \in \Usuff{} | \ \forall y \in \mathcal{Y},  \forall \rv N_i \in \mathrm{Dec}(\rv X, y), \ \rv Z \perp \rv N_i  \  \ \}$ as desired.
\end{proof}



\begin{restatable}[Monotonicity of $\V$-information]{lemma}{monotonicity}\label{lemma:monotonicity}
Let $\V,\mathfam{G} \subseteq \mathcal{P}(\mathcal{Y}|\mathcal{Z})$ 
be two predictive families such that $\V \subseteq \mathfam{G}$, then $\forall \rv Z$ t.v.i $\mathcal{Z}$ and $\forall \rv Y$ t.v.i. $\mathcal{Y}$ we have $\op{I_{\mathcal{G}}}{\rv Z \rightarrow \rv Y} \leq \DIF{Y}{Z}$.
\end{restatable}

\begin{proof}
Let us start from the monotonicity of the predictive entropy \cite{xu2020theory}, which comes directly from the fact that we are optimizing over a larger functional family:
\begin{align*}
\op{H_{\mathcal{G}}}{\rv Y | \rv Z} &\geq \op{H_{\mathcal{G}}}{\rv Y | \rv Z} & \text{Monotonicity $\V$-ent.} \\
\op{H}{\rv Y } - \op{H_{\mathcal{G}}}{\rv Y | \rv Z} &\leq \op{H}{\rv Y } - \op{H_{\mathcal{G}}}{\rv Y | \rv Z} \\
\op{I_{\mathcal{G}}}{\rv Z \rightarrow \rv Y} &\leq \DIF{Y}{Z} & \text{\cref{prop:marginalent}}
\end{align*}
\end{proof}




%%%%%%%%%%%%%%%%%%%%%%%%%%%%%%%%%%%%%%%%%%%%%%
\subsubsection{Optimality of $\V$-Minimality}
\label{appx:proof_optimal}

We will now prove the main result of our paper, namely that any ERM that uses a $\V$-minimal $\V$-sufficient representation will reach the best achievable test loss. 
The main difference with \cref{prop:opt_qsuf} is that the following talks about the optimality of \textit{any} ERMs rather than the existence of at least one such ERM.
Although the proof is relatively long, the intuition is quite simple. Here is a rough outline:

\begin{enumerate}
\item As the theorem is about \textit{all} ERMs, use a proof by contrapositive to only talk about a single ERM $\hat{f}^*$ that performs optimally on train but not on test.
\item Construct a random variable $\tilde{\rv N}$ which labels train examples as 1 and test as 0. Show that $ \tilde{\rv N} \in \decxy{}$
\item Due to the piecewise universality assumption, show that as $\hat{f}^* \in \V$ can distinguish between train and test then there is a $\tilde{f} \in \V$ that can predict $\tilde{\rv N}$ better than random. 
\item Show that it entails $\op{I_{\V}}{\rv Z \to \tilde{\rv N}} \neq 0$. Conclude by \cref{lemma:zeroVminimal} that $\rv Z \not \in \Qsmin{}$ as desired. 
\end{enumerate}


Formally:

\begin{theorem*}\label{theo:opt_qmin_formal} 
Let $\sampleD{}$ be a sampled dataset.
$\rv Z \in \Qsmin{}$  $\implies$  $\forall \hat{f}^* \in \hat{V}^*(\mathcal{D}, \rv Z)$ we have $(\hat{f}^*, \rv Z) \in (\V^*, \rv Z^*)$.
\end{theorem*}

\begin{proof}
For ease of notation we assume that we are in a binary classification setting $|\mathcal{Y}|=2$.
The proof generalizes to the multi-classification setting as well due to the invariance of $\V$ to label permutations.

We will prove the statement by contrapositive, namely $\exists \hat{f}^* \in \hat{V}^*(\mathcal{D}, \rv Z)$ s.t. $(\hat{f}^*, \rv Z) \not \in (\V^*, \rv Z^*)$   $\implies$   $\rv Z \not \in \Qsmin{}$.

The left hand side means that $\exists y \in \mathcal{Y}$ s.t. $\qCH{\hat{f}^*}{Y=y}{Z} \neq \eqCH{\hat{f}^*}{Y=y}{Z}{D} = 0 $.
Due to the deterministic labeling hypothesis and the $\V$-sufficiency of $\rv Z$ (\cref{lemma:VsuffSupp}), we can study one single such label $y$ without considering any other label $y'$ (neither the examples nor the representations interact between labels).

Let $\mathcal{X}^{t}_y$ be the set of examples (associated with $y$) seen during training and  $\mathcal{X}^{e}_y = \mathcal{X}_y \setminus \mathcal{X}^{t}_y$ those only during test (eval). 
Let $\mathcal{Z}^{w}_y \defeq \{ z_y \in \mathcal{Z}_y | \hat{f}^*[z_y](y) \neq 1 \}$ be the set of representation (associated with $y$) who are (wrongly) not given a probability of 1 for the correct label. 
Let $\mathcal{Z}^{c}_y \defeq \mathcal{Z}_y \setminus \mathcal{Z}^{w}_y $ be the set of representations that are (correctly) labeled $y$ by $\hat{f}^*$ with a probability of 1.

Let $\tilde{\rv N} \defeq  \mathds{1}[\rv X_y \in \mathcal{X}^t_y ]$.
I.e. a binary ``selector'' of training examples.
Note that $\tilde{\rv N} \in \decxy{}$, as $\mathds{1}[\cdot \in \mathcal{X}^t_y]$ is a deterministic function from $\mathcal{X}_y \to \mathcal{Y}$.
We will now show that $\op{I}{\rv Z_y \rightarrow \tilde{\rv N} }  \neq 0$.
I.e. $\op{H_{\mathcal{V}}}{\tilde{\rv N} \cond \rv Z_y} < \op{H}{\tilde{\rv N}}$.

\iffalse
First, let us derive $\op{H}{\rv N}$:
\begin{align*}
 - \op{H}{\rv N} 
 &\defeq P_{\tilde{\rv N}}(1) \log  P_{\tilde{\rv N}}(1) + P_{\tilde{\rv N}}(0) \log  P_{\tilde{\rv N}}(0) \\ 
 &=  \sum_{x_y \in \mathcal{X}_y} P_{\tilde{\rv N}, \rv X_y }(1, x_y) \log  P_{\tilde{\rv N}}(1) + 
 \sum_{x_y \in \mathcal{X}_y} P_{\tilde{\rv N}, \rv X_y }(0, x_y) \log  P_{\tilde{\rv N}}(0) \\ 
 &= \sum_{x_y \in \mathcal{X}_y^t} P_{\rv X_y }(x_y) \log  P_{\tilde{\rv N}}(1) + 
 \sum_{x_y \in \mathcal{X}_y^e} P_{\rv X_y }(x_y) \log  P_{\tilde{\rv N}}(0) & \text{Def. } \tilde{\rv N} \\ 
&= \sum_{x_y \in \mathcal{X}_y^t} \sum_{z_y \in \mathcal{Z}_y} P_{\rv X_y, \rv Z_y }(x_y, z_y) \log  P_{\tilde{\rv N}}(1) + 
 \sum_{x_y \in \mathcal{X}_y^e} 
 \sum_{z_y \in \mathcal{Z}_y}
 P_{\rv X_y, \rv Z_y  }(x_y, z_y) \log  P_{\tilde{\rv N}}(0) \\
&= \sum_{x_y \in \mathcal{X}_y^t} \sum_{z_y \in \mathcal{Z}_y^c} P_{\rv X_y, \rv Z_y }(x_y, z_y) \log  P_{\tilde{\rv N}}(1) + 
 \sum_{x_y \in \mathcal{X}_y^e} 
 \sum_{z_y \in \mathcal{Z}_y}
 P_{\rv X_y, \rv Z_y  }(x_y, z_y) \log  P_{\tilde{\rv N}}(0) & \text{ERM} \\
&= \sum_{x_y \in \mathcal{X}_y^t} \sum_{z_y \in \mathcal{Z}_y^c} P_{\rv X_y, \rv Z_y }(x_y, z_y) \log  P_{\tilde{\rv N}}(1)  + 
 \sum_{x_y \in \mathcal{X}_y^e} 
 \sum_{z_y \in \mathcal{Z}_y^c}
 P_{\rv X_y, \rv Z_y  }(x_y, z_y) \log  P_{\tilde{\rv N}}(0) \\
&+ 
 \sum_{x_y \in \mathcal{X}_y^e} 
 \sum_{z_y \in \mathcal{Z}_y^w}
 P_{\rv X_y, \rv Z_y  }(x_y, z_y) \log  P_{\tilde{\rv N}}(0) 
\end{align*}
Where the second to last line comes from the fact that $\hat{f}^*$ is an ERM, so all training examples were given the correct label with probability one to get an empirical risk of zero (\cref{lemma:existperfect}).
\fi

Let us now derive $\op{H_{\mathcal{V}}}{\rv N | \rv Z_y}$. 
Note that due to the piecewise universality assumption, we know that there exists a function $f_{P_{\rv Y}} \in V$ s.t. $\forall z_y \in \mathcal{Z}_y^c$ we have $f_{P_{\rv Y}}[z_y]=P_{\rv Y}$.

Let us denote by $f_c \in V$
\begin{align*}
 - \op{H_{\mathcal{V}}}{\rv N | \rv Z_y } 
 &\defeq 
 \sup_{f \in \V} \biggl(
 \sum_{z_y \in \mathcal{Z}_y}  P_{\tilde{\rv N}, \rv Z_y}(1, z_y) \log  f[z_y](1) \\
 &+ \sum_{z_y \in \mathcal{Z}_y}  P_{\tilde{\rv N}, \rv Z_y}(0, z_y) \log  f[z_y](0) 
 \biggr) \\
 &\geq   
 \sum_{z_y \in \mathcal{Z}_y}  P_{\tilde{\rv N}, \rv Z_y}(1, z_y) \log  f_c[z_y](1) \\
 &+ \sum_{z_y \in \mathcal{Z}_y}  P_{\tilde{\rv N}, \rv Z_y}(0, z_y) \log  f_c[z_y](0) 
  \\
 &= 
 \sum_{z_y \in \mathcal{Z}_y} \sum_{x_y \in \mathcal{X}_y}  P_{\tilde{\rv N}, \rv Z_y,\rv X_y}(1, z_y, x_y) \log  f_c[z_y](1) \\
 &+ \sum_{z_y \in \mathcal{Z}_y} \sum_{x_y \in \mathcal{X}_y}  P_{\tilde{\rv N}, \rv Z_y, \rv X_y}(0, z_y, x_y) \log  f_c[z_y](0) 
  \\
&=  
 \sum_{z_y \in \mathcal{Z}_y} \sum_{x_y \in \mathcal{X}_y^t}  P_{\rv Z_y,\rv X_y}(z_y, x_y) \log  f_c[z_y](1) \\
 &+ \sum_{z_y \in \mathcal{Z}_y} \sum_{x_y \in \mathcal{X}_y^e}  P_{\rv Z_y, \rv X_y}(z_y, x_y) \log  f_c[z_y](0) & \text{Def. }  \tilde{\rv N} 
  \\
&=  
 \sum_{z_y \in \mathcal{Z}_y^c} \sum_{x_y \in \mathcal{X}_y^t}  P_{\rv Z_y,\rv X_y}(z_y, x_y) \log  f_c[z_y](1)  & \text{Def. }  \hat{f}^*,f_c,\mathcal{Z}_y^c  \\
 &+ \sum_{z_y \in \mathcal{Z}_y^c} \sum_{x_y \in \mathcal{X}_y^e}  P_{\rv Z_y, \rv X_y}(z_y, x_y) \log  f_c[z_y](0)   \\
 &+ \sum_{z_y \in \mathcal{Z}_y^w} \sum_{x_y \in \mathcal{X}_y^e}  P_{\rv Z_y, \rv X_y}(z_y, x_y) \log  f_c[z_y](0) \\
 &=  
 \sum_{z_y \in \mathcal{Z}_y^c} \sum_{x_y \in \mathcal{X}_y^t}  P_{\rv Z_y,\rv X_y}(z_y, x_y) \log  P_{\rv X_t | \rv Z_y}( \rv X_t \in \mathcal{X}_y^t | \rv Z_y \in  \mathcal{Z}_y^c) & \text{Set } f_c  \\
 &+ \sum_{z_y \in \mathcal{Z}_y^w} \sum_{x_y \in \mathcal{X}_y^e}  P_{\rv Z_y, \rv X_y}(z_y, x_y) \log 
1 & \text{Set } f_c \\
&= - \op{H}{\tilde{\rv N} \cond \rv Z_y \in  \mathcal{Z}_y^c} & \text{Def. } \tilde{\rv N}\\
&> - \op{H}{\tilde{\rv N} \cond \rv Z_y} & \mathcal{Z}_y^c \neq \varnothing \\
&\geq  - \op{H}{\tilde{\rv N}} & \text{Conditioning} 
\end{align*}

We conclude that $\op{I}{\rv Z_y \rightarrow \tilde{\rv N} }  \neq 0$, so by \cref{lemma:zeroVminimal}, $\rv Z \not \in \Qsmin{}$ which concludes the proof.
\end{proof}

%{\color{red} to do : show that piecewise universality holds for NN with step wise activation}


\subsubsection{$\V$-Minimality $\V$-Sufficiency Properties}
\label{appx:proof_prop}


\Vminsuff*



\begin{proof}$ $
\begin{description}
\item[Monotonicty] From \cref{lemma:zeroVminimal} we know that $\V$-minimal $\V$-sufficient representation satisfy $\forall y \in \mathcal{Y}, \forall \rv N \in \decxy{}$ we have $\DIF{N}{Z_y}=0$.
Following the same steps, we can show that the same holds when both functional family (with respect to which one is minimal and sufficient) are different.
As a result, we know that $\forall y \in \mathcal{Y}, \forall \rv N \in \decxy{}$  : $\op{I_\mathcal{G}}{\rv Z_y \rightarrow \rv N}=0$.
Using the monotonocity of $\V$-information in our setting (\cref{lemma:monotonicity}) we have $0 = \op{I_{\mathcal{G}}}{\rv Z_y \rightarrow \rv N}  \leq  \DIF{N}{Z_y} $.
As $\V$-information is always positive, we conclude that $\forall y \in \mathcal{Y}, \forall \rv N \in \decxy{}$,  $\DIF{N}{Z_y}=0$.
By \cref{lemma:zeroVminimal}, we conclude that $\rv Z$ is $\V$-minimal $\V$-sufficient as desired.
%
\item[Characterization]
As $\DIFxzCy{}$ is an average over a non negative (positivity of $\V$information) $\DIF{N}{Z_y}$ it is equal to zero if and only if all the terms are zero.
Now let $\rv Z \in \Qsuff{}$ be $\V$-sufficient then $\rv Z \in \Qsuff{} \DIFxzCy{} = 0  \iff \rv Z \in \Qsuff{} \forall y \in \mathcal{Y}, \forall \rv N \in \decxy{} \iff \forall \rv Z \in \Qsmin{}$ where the last $\iff$ comes from \cref{lemma:zeroVminimal}.
This concludes the proof.
%
\item[Recoverability]
Using \cref{prop:recsuff} we know that $\Usuff{}=\suff{} \cap \mathcal{Z}$ so the domain of optimization for minimality and $\universal{}$-minimality is the same.
Using \cref{prop:charminsuff} and \cref{prop:charUminUsuff} we only need to show that both characterizations are the same. I.e. $\forall \rv Z \in \Usuff{}$ we have $\rv Z \perp \rv X | \rv Y \iff \rv N_i \perp \rv Z_y, \ \forall \rv N_i \in \mathrm{Dec}(\rv X, y), \forall y \in \mathcal{Y}$.
As a reminder for the following, $\rv Z_y$ and $\rv X_y$  have by definition distribution $P_{\rv X_y} \defeq P_{\rv X | y}$,$P_{\rv Z_y} \defeq P_{\rv Z | y}$. 

($\implies$) Starting from minimality $\rv Z \perp \rv X | \rv Y $ so $\forall y \in \mathcal{Y}$ we have $P_{\rv X_y, \rv Z_y}=P_{\rv X, \rv Z |y}=P_{\rv X | y}*P_{\rv Z |y}=P_{\rv X_y}*P_{\rv Z_y}$ from which we conclude that $\rv Z_y \perp \rv X_y$.
As,  $\rv N_i = t'_i( \rv X_y)$ we also have $\rv Z_y \perp \rv N_i$, $\forall \rv N_i \in \decxy{}$ as desired.\\

($\impliedby$) Let us prove it by contrapositive. I.e. we show that $\rv Z \not \perp \rv X | \rv Y \implies \exists y \in \mathcal{Y}, \exists \rv N_i \in \mathrm{Dec}(\rv X, y) \ s.t. \  \rv N_i \not\perp \rv Z_y $.
As $\rv Z \not \perp \rv X | \rv Y$ then  $\exists \Tilde{x} \in \mathcal{X}, \Tilde{y} \in \mathcal{Y}$ s.t. $P_{\rv Z |\rv X, \rv Y } (\cdot \cond \Tilde{x},\Tilde{y})  \neq P_{\rv Z| \rv Y}(\cdot \cond \Tilde{y})$.
Let us define  $ \tilde{\rv N} = \mathds{1}[\rv X_{\tilde{y}}  = \tilde{x}_{\tilde{y}}] $,
as $\mathds{1}[\rv X_{\tilde{y}}  = \cdot ]$ is a deterministic function from $\mathcal{X}_{\tilde{y}} \to \mathcal{Y}$, we have $\tilde{\rv N} \in \mathrm{Dec}(\rv X, \tilde{y})$.
Then:
\begin{align*}
P_{\rv Z_\tilde{y}| \tilde{\rv N}}(\cdot \cond 1) 
&= P_{\rv Z| \tilde{\rv N}, \rv Y}(\cdot \cond 1, \tilde{y}) & \text{Def. } \rv Z_\tilde{y} \\
&= P_{\rv Z |\rv X, \rv Y } (\cdot \cond \Tilde{x},\Tilde{y}) & \text{Def. }  \tilde{\rv N} \\
&\neq P_{\rv Z| \rv Y}(\cdot \cond \Tilde{y}) & \text{Def. }  \tilde{x},\tilde{y} \\
&= P_{\rv Z_{\tilde{y}}} & \text{Def. }  \rv Z_{\tilde{y}}
\end{align*}
As $P_{\rv Z_{\tilde{y}} | \tilde{\rv N}}(\cdot \cond 1)  \neq P_{\rv Z_{\tilde{y}}}$ we conclude that $\exists \tilde{y} \in \mathcal{Y}, \exists \rv N_i \in \mathrm{Dec}(\rv X, \tilde{y}) \ s.t. \  \rv N_i \not\perp \rv Z_{\tilde{y}} $ as desired.
\end{description}
\end{proof}

\yann{to do corrolary optimality of min suff}
