# Supplementary material for: Learning Optimal Representations with the Decodable Information Bottleneck
Source: arXiv:2009.12789 source file (2021-07-16)
Supplement: Supplementary file 5 [file proof_old.tex]

\section{Theoretical Results and Proofs}

\ydnote{The following has to be a rearranged / cleaned / clarified. I'm currently making sure the proof are correct rather than clear.
}

\subsection{Background}
\label{sec:proof_bckgrnd}

A standard and more detailed review of information theory and probabilistic supervised learning can be found in \citet{cover2012elements} and \citet{gressmann2018probabilistic} respectively.


\begin{restatable}[Strict Properness of Log Loss]{proposition}{properness}\label{prop:proper}
\ydnote{Should remove and simply cite: there's nothigng non standard here}
$\forall x \in \mathcal{X}$ and $\forall Q_{\hrv Y \cond \rv x} \in [\mathcal{X} \to \mathcal{P}(\mathcal{Y})]$ not equal to $P_{\rv Y \cond \rv x}$:
\[\E{y \sim P_{\rv Y \cond \rv x}}{S(y,P_{\rv Y \cond x})} < \E{y \sim P_{\rv Y \cond \rv x}}{S(y,Q_{\hrv Y \cond x})}\]
%We say that the log loss $S$ is a strictly proper scoring rule.
\end{restatable}

%\properness*
\begin{proof}
For notational convenience we use the respective probability mass functions $p,q$ of $P_{\rv Y \cond \rv z=z},Q_{\hrv Y \cond \rv Z=z}$. 

\begin{align*}
\Delta &\defeq 
\E{y \sim P_{\rv Y \cond \rv z=z}}{S(y,Q_{\hrv Y \cond \rv Z=z})} - \E{y \sim P_{\rv Y \cond \rv z=z}}{S(y,P_{\rv Y \cond \rv Z=z})} \\
&= -\sum_{y \in \mathcal{Y}} p(y \cond z) \log q(y \cond z) - \sum_{y \in \mathcal{Y}} -p(y \cond z) \log p(y \cond z) \\
&= \sum_{y \in \mathcal{Y}} p(y \cond z) \log \frac{p(y \cond z)}{q(y \cond z)} & \text{$p,q$ same support}\\
&= \KL{P_{\rv Y \cond \rv z=z},Q_{\hrv Y \cond \rv Z=z}} \\ 
&> 0 & \text{$p \neq q$}
\end{align*}
Where the last line comes from the positive definiteness of the KL divergence when $p \neq q$.
\end{proof}

\begin{restatable}[Data Processing Inequality]{proposition}{dpi}\label{prop:dpi}
If $\rv Y - \rv X - \rv Z$ is a Markov Chain then $ \op{H}{\rv Y \cond \rv Z} \geq \op{H}{\rv Y \cond \rv x}$.
\end{restatable}

%\dpi*
\begin{proof}
By substracting $\op{H}{\rv Y}$ on both sides from the standard DPI \cite{cover2012elements}.
\end{proof}

\begin{restatable}[Invariance to Bijections]{proposition}{bij}\label{prop:bij}
If $f$ is a bijection then $\op{H}{\rv Y} = \op{H}{f(\rv Y)}$ .
\end{restatable}

\begin{proof}
(intuition) change of discrete variable with bijection \ydnote{check : http://www.stat.umn.edu/geyer/f11/5101/notes/n1.pdf, https://www.math.arizona.edu/~jwatkins/f-transform.pdf, https://www.randomservices.org/random/dist/Transformations.html, http://www.math.umd.edu/~millson/teaching/STAT400/slides/article9.pdf}. 
\end{proof}

\begin{corollary}\label{cor:bij}
If $f$ is a bijection then $\op{H}{\rv Z \cond \rv X} = \op{H}{f(\rv Z) \cond \rv X}$ and $\op{H}{\rv X \cond \rv Z} = \op{H}{\rv X \cond  f(\rv Z)}$.
\end{corollary}

\begin{proof}
Letting $\rv Y = (\rv Z, \rv X)$ in \cref{prop:bij} we have $\op{H}{\rv Z,\rv X} = \op{H}{f(\rv Z ,\rv X)}$ for any bijection. Let $g$ also be a bijection, then $f(\cdot)=(g(\cdot),\cdot)$ is a bijection and we thus have $\op{H}{\rv Z,\rv X} = \op{H}{g(\rv Z),\rv X}$ substracting $\op{H}{\rv X}$ both sides we get $\op{H}{\rv Z \cond  \rv X} = \op{H}{g(\rv Z) \cond \rv X)}$. By the same argument with a bijection $g'$ and letting $f(\cdot)=(\cdot,g'(\cdot))$ we get $\op{H}{\rv X \cond  \rv Z} = \op{H}{g'(\rv X) \cond \rv Z}$ which concludes the proof.
\end{proof}

Note that the previous proposition and corollary only hold because of our simplifying assumption of finite sample spaces. 
In the case of continuous r.v., it is nevertheless possible to show that if $f$ is a homeomorphism (i.e. smooth bijection) then $\op{H}{\rv X \cond \rv Z} = \op{H}{\rv X \cond  f(\rv Z)}$. This can be proven by the invariance of mutual information to homeomorphisms \cite{kraskov2004estimating}.
So the intuition that we give in the main text of conditional entropy not being the right measure for the quality of a representation still holds for continuous r.v. as one could entangle representations in a very non linear fashion without affecting conditional entropy.

In the following, we will prove the equivalence between our definition of (minimal) sufficient statistics and the standard ones.
Note that in the main text we allow ourselves to work with stochastic representations. 
This contrasts with the definition of statistic, namely that a statistic $\rv Z$ of $\rv X$ is any composition between a measurable function $E$ and $\rv X$ (essentially deterministic representations).
As standard minimality and sufficiency is not defined for ``stochastic statistics'', we only show the equivalence for deterministic statistics.
\ydnote{Here I only prove the equivalence with predictive sufficient statistics which recovers the usual sufficient statistics if $\rv Y = \Theta$ \tocite{}}

\begin{definition}[Standard Sufficient Statistic]\label{def:standard_sufficiency}
A statistic $\rv Z$ of $\rv X$ is said predictive sufficient for $\rv Y $ if $\rv Y - \rv Z - \rv X$ forms a Markov Chain.
\end{definition}

\begin{proposition}[Equivalence of Sufficient Statistics]
Let $\rv Y, \rv X$ be two random variables, and $E$ a deterministic function.
A statistic $\rv Z \defeq E(\rv X)$ of $\rv X$ is predictive sufficient for $\rv Y$ by \cref{def:standard_sufficiency} if and only if it is sufficient for $\rv Y$ by \cref{def:predictive_min}.
\end{proposition}

\begin{proof}
First, assume that $\rv Z$ is sufficient by \cref{def:standard_sufficiency}. Namely, $\rv Y - \rv X - \rv Z$ constitutes a Markov Chain.
From the data processing inequality (DPI) we have $\MI{Y}{X} \geq \MI{Y}{Z}$. Since $\rv Z$ is sufficient, we also have $\rv Y - \rv Z - \rv X $. Using again the DPI, we have $\MI{Y}{Z} \geq  \MI{Y}{X}$. Due to the upper and lower bound we must have $\MI{Y}{X} = \MI{Y}{Z}$. This can be further decomposed as $\op{H}{\rv Y} - \op{H}{\rv Y \cond \rv X} = \op{H}{\rv Y} - \op{\rv H}{\rv Y \cond \rv Z}$, from which we conclude that $\op{H}{\rv Y \cond \rv X} = \op{H}{\rv Y \cond \rv Z}$.

For the second direction, assume that $\rv Z$ is sufficient by \cref{def:predictive_min}. 
 Using the chain rule of information we have 
 \begin{align*}
\MI{Y}{Z,\rv X} &= \MI{Y}{Z ,\rv X}\\
\MI{Y}{Z}+\MI{Y}{X \cond \rv Z}&=\MI{Y}{X}+\MI{Y}{Z \cond \rv X}\\
\op{H}{\rv Y} - \op{H}{\rv Y \cond \rv Z} +\MI{Y}{X \cond \rv Z} &= \op{H}{\rv Y}- \op{H}{\rv Y \cond \rv X} +\MI{Y}{Z \cond \rv X}\\
- \op{H}{\rv Y \cond \rv Z} +\MI{Y}{X \cond \rv Z} &=- \op{H}{\rv Y \cond \rv X} +\MI{Y}{Z \cond \rv X}\\
- \op{H}{\rv Y \cond \rv Z} +\MI{Y}{X \cond \rv z}&=- \op{H}{\rv Y \cond \rv Z} +\MI{Y}{Z \cond \rv X} & \text{\cref{def:predictive_min}}\\
\MI{Y}{X \cond \rv z}&= \MI{Y}{z \cond \rv X} \\
\MI{Y}{X \cond \rv z}&= 0 & \rv Y - \rv X - \rv Z \\
 \end{align*}
 
 Where the last line used the fact that $\rv Z$ is a statistic of $\rv X$.  
 $\MI{Y}{X \cond Z}= 0$, implies that $\rv Y - \rv Z - \rv x$ is a Markov chain, which concludes the proof.
\end{proof}

\begin{definition}[Standard Minimal Sufficient Statistic]\label{def:standard_minimality}
A sufficient statistic $\rv Z$ of $\rv X$ for $\rv Y$ is said \textit{minimal} if for any other sufficient statistic $\rv Z'$ of $\rv X$ for $\rv Y$, there exists a measurable function $g$ such that $\rv Z = g(\rv Z')$ almost everywhere.
\end{definition}

\begin{proposition}[Equivalence of Sufficient Statistics]
Let $\rv Z$ denote a \textit{sufficient} statistic of $\rv X$ for $\rv Y$.
Then it is called minimal by  \cref{def:standard_minimality} if and only if it is minimal by \cref{def:predictive_min}.
\end{proposition}

\begin{proof}
 Let $\rv Z$ be minimal by \cref{def:standard_minimality}, then $\forall \rv Z' \in \suff{}$ we have  the Markov Chain $\rv X - \rv Z' - \rv Z $. 
 From the DPI, $\op{H}{\rv X} - \op{H}{\rv X \cond \rv Z} = \MI{X}{Z} \leq \MI{ X}{Z'} = \op{H}{\rv X} - \op{H}{\rv X \cond \rv Z'}$. Rearranging we have $\op{H}{\rv X \cond \rv Z} \geq \op{H}{\rv X \cond \rv Z'}$. This completes the first direction of the proof.
 
For the other direction, suppose $\rv Z \defeq E(\rv X)$ is not minimal by \cref{def:standard_minimality}, i.e. there exists a sufficient statistic $\rv Z' \defeq E'(\rv X)$ such that there is no function $g$ that satisfies $f(\rv X) = g(E'(\rv X))$. 
Then the binary relation $\{(E'(x), E(x)) \cond x \in \mathcal{X}\}$ is not univalent, therefore the converse relation $\{(E(x),E'(x)) \cond x \in \mathcal{X}\}$ is not injective.
As a result, there exists a non injective function $\Tilde{g}$ such that
$E'(\rv X) = \Tilde{g}(E(\rv X))$. 
From the DPI we have $\op{H}{\rv X} - \op{H}{\rv X \cond \rv Z'} = \MI{X}{Z'} < \MI{ X}{Z} = \op{H}{\rv X} - \op{H}{\rv X \cond \rv Z}$ with a strict inequality due to the non injectivity of $\Tilde{g}$.
In summary, we supposed $\rv Z$ was not minimal by \cref{def:standard_minimality} and found that $\op{H}{\rv X \cond \rv Z} < \op{H}{\rv X \cond \rv Z'}$ meaning that $\rv Z$ is not minimal by \cref{def:predictive_min}.
By contrapositive, we conclude that minimality by \cref{def:predictive_min} implies minimality by \cref{def:standard_minimality}, thus concluding the proof.
\end{proof}



\subsection{Conditional Entropy}
\label{sec:proof_dif}

%FOr reasons 

%In this section we will discuss why the decodable entropy is defined as it is and what are the properties it satisfies.
%Conditional entropy is a well studied operator that has many desirable properties \tocite{} and is fundamental for information theory (as mutual information can be decomposed in an entropy and conditional entropy term). 
%We strongly believe that it is useful but have argued in the main text that it is is not completely satisfactory as it does not take into account the functional family at hand.
%The main issue is that it is defined using the underlying conditional distribution, which might not be available in a given constrained functional family.
%Due to the strict properness of the log loss \tocite{} we know7 that the underlying conditional distribution is optimal, and as a result would like the notion of decodable entropy to recover conditional entropy when it is not constrained. 
%We will call this property \textbf{weak recoverability}

%\begin{lemma}\label{lem:bij}
%$\op{H}{\rv X \cond \rv Z} = \op{H}{\rv Y \cond \rv Z} \forall \rv Z$ if and only if there exists a bijection $f$ s.t. $\rv X = f(\rv Y)$.
%\end{lemma}
%\begin{proof}
%(intuition) if a bijection exists then $\op{H}{\rv X \cond \rv Z} = \op{H}{\rv Y \cond \rv Z} \forall %\rv Z$ because of the discrete change of variable with a bijection \ydnote{check : http://www.stat.umn.edu/geyer/f11/5101/notes/n1.pdf, https://www.math.arizona.edu/~jwatkins/f-transform.pdf, https://www.randomservices.org/random/dist/Transformations.html, http://www.math.umd.edu/~millson/teaching/STAT400/slides/article9.pdf}.

%(intuition) For the second direction, suppose $\op{H}{\rv X \cond \rv Z} = \op{H}{\rv Y \cond \rv Z} \forall \rv Z$ then we also have that it is true for $\rv Z = \rv Y$ in other words $\op{H}{\rv X \cond \rv Y}=\op{H}{\rv Y \cond \rv Y}=0$ meaning that there exists a function $f$ s.t. $\rv X = f(\rv Y)$. 
%Using the same argument for $\rv Z = \rv X$, we get that $\op{H}{\rv Y \cond \rv X}=\op{H}{\rv X \cond \rv X}=0$ so there exists a function $f^{-1}$ s.t. $\rv Y = f^{-1}(\rv X)$. Putting both equations together we have $\rv Y = f^{-1}(f(\rv Y))$ so $f$ is a bijection.
%\end{proof}


\begin{definition}[Decomposition of Random Variables]\label{def:decomp}
A collection of r.v. $\rv N=\{\rv N_i\}_i$ is a $\mathcal{Y}$ decomposition of a on constant $\rv X$.
If 
\begin{itemize}
\item \textbf{Take value in $\mathcal{Y}$}. Each $\rv N_i \in \rv N$ t.v.i in a set $\mathcal{N}$ whose support is a subset of $\mathcal{Y}$ : $\mathrm{supp}(\mathcal{N}) \subseteq \mathcal{Y}$. 
\item \textbf{Bijection} There exists a bijection $f$ s.t. $\rv X = f(\rv N)$;
\item \textbf{Independence} $\rv N_i \perp \rv N_j, \ \forall \rv N_i \in \rv N \neq \rv N_j \in \rv N$.
\item \textbf{Not Constant} There are no constant r.v. $\rv N_i$.
\end{itemize}
\end{definition}

\begin{restatable}[General Decodable Entropy]{definition}{gen_decentropy}\label{def:gen_q_entropy}
The decodable entropy of $\rv X$ (regardless of its sample space $\mathcal{X}$) conditioned on $\rv Z$ with respect to $\family{} \in [\mathcal{Z} \to \mathcal{P}(\mathcal{Y})]$, is:
\[
\CHF{X}{z} 
\defeq \E{\rv N \sim \mathrm{dec}_{\mathcal{Y}}(\mathcal{X})}{\sum_{N_i \in \rv N}\CHF{N_i}{Z}}
\]
Where $\mathrm{dec}_{\mathcal{Y}}(\rv X)$ is the set of all $\mathcal{Y}$ decompositions of $\mathcal{X}$.
\end{restatable}

In the main body, we gave a slightly different definition which is equivalent but more computationally efficient to work with in the considered task. It uses the base $\mathcal{Y}$ expansion of $\rv X$ instead of the $\mathcal{Y}$ decompositions of $\rv X$.

\expansion*

\begin{restatable}[Decodable Entropy]{definition}{decentropy}\label{def:q_entropy}
The decodable entropy \footnote{A more general definition that encompasses any $\rv X$ under a single equation is discussed in \cref{sec:proof_dif}. Although more general it is slightly more difficult to understand and not useful for our setting. Indeed, in machine learning one always samples a dataset from a distribution, so the empiricial random variable can always be rewritten as a uniform random variable over indices of the dataset.} of $\cdot$ conditioned on $\rv Z$ with respect to $\family{} \in [\mathcal{Z} \to \mathcal{P}(\mathcal{Y})]$, is:
\begin{itemize}
\item \textbf{Simple Case} if $\cdot=\rv Y$ t.v.i $\mathcal{Y}$
\[
\CHF{y}{z} 
\defeq 
\inf_{Q \in \mathfam{Q}} \E{n_i,z \sim P_{\rv N_i \times \rv z}}{S(n_i,\pred{}))} 
\]
\item \textbf{Complex Case} if $\cdot=\rv X$ t.v.i. $\mathcal{X} \neq \mathcal{Y}$ and with distribution $P_{\rv X}=\mathrm{Unif}(\mathcal{X})$. Let $(\rv N_i)_i$ be a base $|\mathcal{Y}|$ expansion of $\rv X$ then 
\[
\CHF{X}{z} 
\defeq \sum_{i=0}^{\ceil{\log_{|\mathcal{Y}|}(|\mathcal{X}|)}-1} \CHF{N_i}{Z}
\]
\end{itemize}
%Where $\rv N_i$ is the $i^{th}$ coefficient of the base $|\mathcal{Y}|$ expansion of a predefined $\mathrm{ind}(x)$. \ydnote{This is not well explained, but I don't know how to do it a more clear fashion. Hopefully the previous paragraph makes it clear though.}
\end{restatable}

Importantly, both definitions are equivalent for the considered cases as we will now show.

\begin{lemma}\label{lem:expansion_decomposition}
Let $|\mathcal{Y}|=[0,\dots,|\mathcal{Y}|-1]$, then any base $|\mathcal{Y}|$ expansion of a $\mathcal{X}$ with uniform distribution $P_{\rv X}=\mathrm{Unif}(\mathcal{X})$ is also a $\mathcal{Y}$ decomposition of $\rv X$.
\end{lemma}
\begin{proof}
\item \textbf{Take value in $\mathcal{Y}$}. Let $\rv N = (\rv N_i)_i$ be a base $|\mathcal{Y}|$ expansion of $\mathcal{X}$, then by definition  $\forall \rv N_i$ there exists $f_i : \mathcal{X} \to [0, \dots ,|\mathcal{Y}|-1]$ s.t. $\rv N_i = f_i(\rv X)$. Due to our multi-class classification assumption, $\mathcal{Y}=[0, \dots ,|\mathcal{Y}|-1]$ from which we conclude that $\rv N_i$ t.v.i $\mathcal{Y}$.
\item \textbf{Bijection}  Let $f^{-1} : \mathcal{Y}^{\ceil{\log_b{\mathcal{X}}}-1} \to [0, \dot ,|\mathcal{X}|-1]$ a function that maps $\rv N \mapsto \sum_{i=0}^{\ceil{\log_b{\mathcal{X}}}-1} \rv N_i b^{i}$.
Applying it to the base $|\mathcal{Y}|$ expansion of $\mathcal{X}$ :  $\rv N = (\rv f_i(\rv X))_i$ we get $\forall x \in \mathcal{X}$:
\begin{align*}
f^{-1}((\rv f_i(x))_i) 
&= \sum_{i=0}^{\ceil{\log_b{\mathcal{X}}}-1} f_i(x) b^{i} \\
&= \mathrm{ind}(x)  \\
\mathrm{ind}^{-1}f^{-1}((\rv f_i(x))_i)  &= x & \text{Def. Property}  \\
\end{align*}
Where the last line comes from the defining property of a $|\mathcal{Y}|$ expansion of $\mathcal{X}$ which ensures that $\mathrm{ind}$ is a bijection, and thus invertible as both sides of the equality are defined on $[0, \dot ,|\mathcal{X}|-1]$. Putting all together we get that $g=\mathrm{ind}^{-1}f^{-1}$ is a bijection and $\rv X = g(\rv N)$.
\item \textbf{Independence} .
\item \textbf{Not Constant} .
\end{proof}


\begin{proposition}
\cref{def:q_entropy} is equivalent to \cref{def:gen_q_entropy} for the two cases that are considered.
\end{proposition}
\begin{proof} 
\hfill
\begin{itemize}
\item \textbf{Simple Case} Let $\rv Y$ t.v.i $\mathcal{Y}$ and $\CHF{y}{z}$ be as defined in \cref{def:gen_q_entropy}, then :
\begin{align*}
\CHF{X}{z} 
&\defeq \E{\rv N \sim \mathrm{dec}_{\mathcal{Y}}(\rv X)}{\sum_{N_i \in \rv N}\CHF{N_i}{Z}} \\
&= \E{\rv N \sim \mathrm{dec}_{\mathcal{Y}}(\rv X)}{\CHF{N_0}{Z}} & \text{Singleton $\rv N$} \\
&= \E{f \sim \{f' \in [\mathcal{Y} \to \mathcal{Y}] \ s.t. \ f' \text{is a bijection} \} }{\op{H}{f(\rv N_0),\rv Z}} & \text{Bijection} \\
&= \CHF{Y}{Z} & \text{Inv. to Perm.} \\
\end{align*}
Where the second line used the fact that the number of $\rv N_i \in \rv N$ has to be $m=1$. 
Indeed, by the definition of a $\mathcal{Y}$ decomposition of $\rv Y$ there needs to be a bijection between $\rv N$ and $\rv Y$ meaning that the cardinality of their respective sample space has to be equal. 
The cardinality the sample space of $\rv N$ is $|\mathcal{N}|=|\mathcal{Y}|^m$  --- each $\rv N_i$ is non constant and t.v.i $\mathcal{Y}$ --- so $m=1$ to satisfy $|\mathcal{N}|=|\mathcal{Y}|^m=|\mathcal{Y}|$.
The third line used the fact that if $m=1$ then the set of all decompositions $\mathrm{dec}_{\mathcal{Y}}(\rv Y) = \{f(\rv Y) \ s.t. \ f \text{vis a permutation of } \rv Y \}$, where a permutation is a bijection where the domain and codomain coincide.
The last line used the invariance of the predictive family $\family{}$ to permutations.
%%%
\item \textbf{Complex Case} Let $\rv X$ t.v.i. $\rv X$ t.v.i. $\mathcal{X} \neq \mathcal{Y}$ with distribution $P_{\rv X}=\mathrm{Unif}(\mathcal{X})$ and $\CHF{x}{z}$ be as defined in \cref{def:gen_q_entropy}, then :
\begin{align*}
\CHF{X}{z} 
&\defeq \E{\rv N \sim \mathrm{dec}_{\mathcal{Y}}(\rv X)}{\sum_{N_i \in \rv N}\CHF{N_i}{Z}} \\
&= \E{\rv N \sim \mathrm{dec}_{\mathcal{Y}}(\rv X)}{\CHF{N_0}{Z}} & \text{Singleton $\rv N$} \\
&= \E{f \sim \{f' \in [\mathcal{Y} \to \mathcal{Y}] \ s.t. \ f' \text{is a bijection} \} }{\op{H}{f(\rv N_0),\rv Z}} & \text{Bijection} \\
&= \CHF{Y}{Z} & \text{Inv. to Perm.} \\
\end{align*}
Where the f
\end{itemize}
\end{proof}










\begin{lemma}[Decomposition and Weak Recoverability]\label{lem:weak}
Let $\rv N = ( \rv N_i )_i$ be a random vector with component $\rv N_i$ then $\sum_{\rv N_i \in \rv N } \inf_{U \in \mathfam{U}} \E{n_i,z \sim P_{\rv N_i \times \rv z}}{S(n_i,U_{\hrv N_i \cond z}))} = \op{H}{\rv X \cond \rv Z }$ $\forall \rv Z$ if and only if $\rv N$ is a $\mathcal{Y}$ decomposition of $\rv X$.
\end{lemma}

\begin{proof}
\begin{description}
\item[Take value in $\mathcal{Y}$] Suppose $\exists i \ s.t. \ \rv N_i$ does not satisfy the $\mathcal{Y}$-requirement. Then there exists $n_i \not\in \mathcal{Y}$, which happens with non zero probability. As a result, $S(n_i,U_{\hrv N_i \cond z}))=- \log(U_{\hrv N_i \cond z}(n_i \cond z))$ is not well defined (because the codomain of $U_{\hrv N_i \cond z}$ is wrong) . The expectation over $\rv N_i$ is thus also not well defined (as $U$ t.v.i in $\mathcal{P}(\mathcal{Y})$ ).
\item[Bijection and Independence] 
First let us show that if $\rv N$ is a $\mathcal{Y}$ decomposition of $\rv X$ , then $\sum_{\rv N_i \in \rv N } \inf_{U \in \mathfam{U}} \E{n_i,z \sim P_{\rv N_i \times \rv z}}{S(n_i,U_{\hrv N_i \cond z}))} = \op{H}{\rv X \cond \rv Z }$:
\begin{align*}
\op{\Tilde{H}_{\mathfam{U}}}{\rv X \cond \rv Z} &= \sum_{\rv N_i \in \rv N } \inf_{U \in \mathfam{U}} \E{n_i,z \sim P_{\rv N_i \times \rv z}}{S(n_i,U_{\hrv N_i \cond z}))} \\
&= \sum_{\rv N_i \in \rv N } \E{n_i,z \sim P_{\rv N_i \times \rv z}}{S(n_i,P_{\hrv N_i \cond  z}(n_i \cond z)} & \text{Strictly Proper} \\
&= \sum_{\rv N_i \in \rv N } \op{H}{\rv N_i \cond \rv Z} & \text{Definition} \\
&= \op{H}{(\rv N_i)_i \cond \rv Z} & \text{Independence} \\
&= \op{H}{f((\rv N_i)_i) \cond \rv Z} & \text{\cref{cor:bij}} \\
&= \op{H}{\rv X \cond \rv Z} 
\end{align*}
Where the second line uses the strict properness of the log loss and the fact that $P_{N_i \cond \rv z} \in [\mathcal{Z} \to \mathcal{P}(\mathcal{Y})] \eqdef \universal{}$. 
Where the last line comes from the assumption that there exists a bijection $f$ s.t. $\rv X = f(\rv N)$.
This proves the first direction. 

For the other direction , suppose that $\sum_{\rv N_i \in \rv N } \inf_{U \in \mathfam{U}} \E{n_i,z \sim P_{\rv N_i \times \rv z}}{S(n_i,U_{\hrv N_i \cond z}))} = \op{H}{\rv X \cond \rv Z }$ $\forall \rv Z$.
Using the strict properness of the log loss (as before) we get that $\sum_{\rv N_i \in \rv N } \op{H}{\rv N_i \cond \rv Z} = \op{H}{\rv X \cond \rv Z}, \ \forall Z$.

Set $\rv Z = \rv X$ then $\sum_{\rv N_i \in \rv N } \op{H}{\rv N_i \cond \rv X} = \op{H}{\rv X \cond \rv X} = 0$. 
As conditional entropy is non-negative (discrete case), then we must have $\op{H}{\rv N_i \cond \rv X}=0, \ \forall i$. From which we conclude that $\forall i$ there exists $f_i$ s.t. $\rv N_i = f_i(\rv Z)$.
Similarly set $\rv Z = \rv N$ then $\op{H}{\rv N_i \cond \rv N}=0, \ \forall N_i \in \rv N$ so $\op{H}{\rv X \cond \rv N } = \sum_{\rv N_i \in \rv N } \op{H}{\rv N_i \cond \rv X} = 0$ from which we conclude that there is a function $f^{-1}$ s.t. $\rv X = f^{-1}(\rv N)$. 
Putting it with the previous equation we have $\rv X = f^{-1}(\rv N) = f^{-1}((\rv N_i)_i) =  f^{-1}(( f_i(\rv X) )_i)$ from which we conclude that $f(\cdot)=(f_i(\cdot))_i$ is a bijection.

Finally, suppose $\rv Z$ is independent of $\rv X$. As there exists a bijection between $\rv N$ and $\rv X$ we also have that $\rv Z \perp \rv N$ so
\begin{align*}
\op{H}{\rv X } 
&= \op{H}{\rv X \cond \rv Z} & \rv Z \perp \rv X \\
&= \sum_{\rv N_i \in \rv N } \op{H}{\rv N_i \cond \rv Z} & \text{Supposition} \\
&= \sum_{\rv N_i  } \op{H}{\rv N_i} & \rv Z \perp \rv N \\
&\geq \op{H}{(\rv N_i)_i }  \\
&= \op{H}{f((\rv N_i)_i)} & \text{\cref{cor:bij}} \\
&= \op{H}{\rv X } 
\end{align*}
Obviously $\op{H}{\rv X } = \op{H}{\rv X} $ so the inequality has to be an equality $\sum_{\rv N_i } \op{H}{\rv N_i} = \op{H}{(\rv N_i)_i }$. I.e. $\rv N_i \perp \rv N_j, \forall i \neq j$, which concludes the proof.
\end{description}
\end{proof}

It has the following desirable properties

\propentropy*
\begin{proof}
\begin{description}
%\item[Positivity] The log score is non-negative  $S(n_i,\pred{}) = - \log Q(n_i|\rv Z) \geq 0$ and expectations, infimums, and sums preserve non-negativity. Note that this only holds because discreteness assumptions of r.v (finite sample spaces). 
%\item[Independence] By the independence property of conditional entropy $\op{H}{\cdot \cond \rv z} = \op{H}{\cdot}$ if and only if $\cdot \indep \rv z$.
\item[Monotonicity] Let $\family{} \subseteq \pFam{\mathfam{G}}$, $\mathcal{A}_i \defeq \{\E{n_i ,z \sim P_{\rv N_i \times \rv z}}{S(n_i,\pred{}))} \ s.t. \ \pred{} \in \family{} \}$, and $\mathcal{B}_i \defeq \ \{\E{n_i,z \sim P_{\rv N_i \times \rv Y}}{S(n_i,\pred{}))} \ s.t. \ \pred{} \in \pFam{\mathfam{G}} \}$.
The image of a subset under a mapping is the subset of the image, so we have $\mathcal{A}_i \subseteq \mathcal{B}_i$.
By the subset property of infimums $\mathcal{A}_i \subseteq \mathcal{B}_i$ implies $\inf \mathcal{A}_i \geq \inf \mathcal{B}_i$, $\forall i = 0, \dots, \ceil{\log_{|\mathcal{Y}|}(|\mathcal{X}|)}-1$.
As the previous inequality holds for all $i$, we have that the inequality also holds for the sum of all terms : $\CHF{X}{Z} = \sum_{0}^{\ceil{\log_{|\mathcal{Y}|}(|\mathcal{X}|)}-1} \inf \mathcal{A}_i \geq \sum_{0}^{\ceil{\log_{|\mathcal{Y}|}(|\mathcal{X}|)}-1} \inf  \mathcal{B}_i = \op{H_{\mathfam{G}}}{\rv X, \rv Z}$. 
\item[Weak Recoverability] We want to show $\op{H}{\rv X \cond \rv z} =  \op{H_{\mathfam{U}}}{\rv X \cond \rv z} \defeq \sum_{i=0}^{\ceil{\log_{|\mathcal{Y}|}(|\mathcal{X}|)}-1} \inf_{U \in \mathfam{U}} \E{n_i,z \sim P_{\rv N_i \times \rv z}}{S(n_i,U_{\hrv N_i \cond z}))}$. Given the form of the last equation, we can apply \cref{lem:weak}, which stipulates that the weak recoverability property is satisfied if and only if $(\rv N_i)_i$ is a $\mathcal{Y}$ decomposition of $\mathcal{X}$.
By definition $(\rv N_i)_i$ is a base $|\mathcal{Y}|$ expansion of $\rv X$, so we just need to show that it implies 
\item[Strong Recoverability]
Note that from the strict properness of the log loss, $\forall \rv Z$ and $\forall \hat{Q}_{\rv Y \cond \rv z} \neq P_{\rv Y \cond \rv z}$, we have:
\begin{align}
\E{y \sim P_{\rv Y \cond \rv z}}{S(y,P_{\rv Y \cond z})} &< \E{y \sim P_{\rv Y \cond \rv z}}{S(y,Q_{\hrv Y \cond z})} \nonumber \\
 \op{H}{\rv Y \cond \rv z} \defeq \E{y,z \sim P_{\rv Y \rv z}}{S(y,P_{\rv Y \cond z})} &< \E{y,z \sim P_{\rv Y \rv z}}{S(y,Q_{\hrv Y \cond z})} \label{eqn:expected_proper}  
\end{align}
For the first direction of the proof, suppose that $P_{\rv Y \cond \rv Z} \in \family{}$ but $\op{H}{\rv Y \cond \rv z} \neq \CHF{y}{z}$. 
Then either $\op{H}{\rv Y \cond \rv z} > \CHF{y}{z}$ or $\op{H}{\rv Y \cond \rv z} < \CHF{y}{z}$.
The former contradicts 
For the second part of the proof, we have to use our assumptions of finite sample sets $\mathcal{Z}$
This comes directly from the properness of log loss (\cref{prop:proper}).
$P_{\rv Y \cond \rv Z} \in \family{}$ if and only if $\op{H}{\rv Y \cond \rv X} =  \CHF{y}{x}$. 
\end{description}


\textbf{Recoverability}: \yann{NOT FINISHED !}
Note that from the strict properness of the log loss, $\forall \rv Z$ and $\forall \hat{Q}_{\rv Y \cond \rv z} \neq P_{\rv Y \cond \rv z}$, we have:
\begin{align}
\E{y \sim P_{\rv Y \cond \rv z}}{S(y,P_{\rv Y \cond z})} &< \E{y \sim P_{\rv Y \cond \rv z}}{S(y,Q_{\hrv Y \cond z})} \nonumber \\
 \op{H}{\rv Y \cond \rv z} \defeq \E{y,z \sim P_{\rv Y \rv z}}{S(y,P_{\rv Y \cond z})} &< \E{y,z \sim P_{\rv Y \rv z}}{S(y,Q_{\hrv Y \cond z})} \label{eqn:expected_proper}  
\end{align}

For the first direction of the proof, suppose that $P_{\rv Y \cond \rv Z} \in \family{}$ but $\op{H}{\rv Y \cond \rv z} \neq \CHF{y}{z}$. 
Then either $\op{H}{\rv Y \cond \rv z} > \CHF{y}{z}$ or $\op{H}{\rv Y \cond \rv z} < \CHF{y}{z}$.
The former contradicts 

For the second part of the proof, we have to use our assumptions of finite sample sets $\mathcal{Z}$

This comes directly from the properness of log loss (\cref{prop:proper}).
$P_{\rv Y \cond \rv Z} \in \family{}$ if and only if $\op{H}{\rv Y \cond \rv X} =  \CHF{y}{x}$. 

\end{proof}


In this section we will show that 

Intuitively, the decomposition should be such that
\begin{inlinelist}
\item $\rv N_i$ t.v.i $\mathcal{Y}$ thus having a well defined $\CHF{N_i}{Z}$;
\item the collection $\rv N$ has all (and only) the information in $\rv X$;
%I.e. we want $\op{H}{\rv X} = \op{H}{\rv N_1, \dots, \rv N_n} = \op{I}{\rv X;\rv N_1, \dots, \rv N_n}$.
\item all $\rv N_i$ should ``carry'' different information about $\rv X$, thus keeping $|\rv N|$ small and avoiding unnecessary computation.
%I.e. all $N_i$ should be independent of each other.
\end{inlinelist}


The exact requirements for the decomposition to be valid are formalized in the following definitions.

\begin{definition}[Decomposition of Random Variables]
A collection of r.v. $\rv N=\{\rv N_i\}_i$ is a $\mathcal{Y}$ decomposition of $\rv X$.
If 
\begin{inlinelist}
\item $\forall \rv N_i \in \rv N, \ \exists $ a function $f_i : \mathcal{X} \to \mathcal{Y}$ s.t. $\rv N_i = f_i(\rv X)$;
\item $\exists f^{-1}$ s.t. $\rv X = f^{-1}(\rv N)$;
\item $\rv N_i \perp \rv N_j, \ \forall \rv N_i \in \rv N \neq \rv N_j \in \rv N$.
\end{inlinelist}
\ydnote{Maybe a little dense in math symbols. I can use more space, use more English word, but I think that the previous paragraph does most of the job on the intuition. Although the definition is important to understand the definition of $\CHF{N_i}{Z}$ it is not crucial to understand in practice as we will only use a very specific decomposition (the minimal one). }
\end{definition}

The smallest set of 


$\family{} \subseteq \pFam{\mathfam{G}}$ then $\CHF{y}{z} \geq \op{H_\mathfam{G}}{\rv Y \cond \rv z}$ 

\propDI*
\begin{proof}
\yann{\textbf{Recoverability} : Already proved recoverablity for predictive entropy, so has to only do it for uninformative. If the underlying marginal is in the proper predictive family, this means that $\exists z$ s.t. $Q_{\rv Y \cond z}=P(\rv Y)$. In other words the marginal is in the range of the family. By definition of a predictive family it means that there's a predictor that will output the marginal regardless of the input. As log loss is proper scoring, this is the best achievable => inf.
\textbf{Independence} : If Independence then by definition, product of marginals is equal to joint => get 0 as the predictive entropy becomes the uninformative one. 
\textbf{Non negativity} :  Unconditional is weighted average (expectation over x) of conditional cross entropy, so to minimize it will chose a predictor which constantly predicts the minimal cross entropy. Because the family is proper, the informed predictive entropy could also predict the same marginal => at least as good.
}
\end{proof}

\subsection{Learning Optimal Representations}

%\sufficiencies*
\begin{proof}
\yann{Last equality comes directly from the definition. First inclusion is trivially true if $\mathcal{S}_{\mathcal{Q}}$ is empty. If it is not empty, it comes from the fact that any $Q_{\rv Y \cond \rv Z=z}$ would by definition be $P_{\rv Y \cond \rv X=x}$. This will usually only be a subset as any ``any bijection applied to Z which cannot be inverted by Q would be sufficient but not Q-sufficient''. Second inclusion comes from the fact that $\mathcal{G} \subseteq \mathcal{U}$.}
\end{proof}


\qminimallink*
\proof{
\begin{itemize}
\item \textbf{Rademacher Complexity}
First let us prove that any $\family{}$-sufficient statistic, which yields the minimum Rademacher complexity is a minimal $\family{}$-sufficient statistic. 
\end{itemize}
}

%%%%%%%%%%%%%%%%
\subsection{$\mathcal{Q}$-Decodable Information Bottleneck}



\optimalqib*

\begin{proof}\label{proof:qib}
\yann{HAS TO BE UPDATED FOR THE NEW DEFINITION + GENERALIZED }

First, let us assume that we have access to an oracle that gave us $q(\rv Y \cond \rv Z)$ and $q'(\rv Y \cond \varnothing)$ as defined in \cref{eqn:q_yz}. 
Important variational derivatives are \footnote{For simplicity, we will use the following abuse of notation $\int_{ Z} z p(z) \defeq \int  Z(w) P(\sd{w})$.
Note that we are integrating over the underlying measure, such that the derivation holds for any distributions (continuous or not).}:

\begin{align*} 
%%%%%%%%%
\partial_{\rv z \to \rv y} 
&\defeq
\frac{\partial}{\partial p(z \cond x) } \op{DI_{\mathcal{Q}}}{ Z \to  Y}
\nonumber  \\
%
&= \frac{\partial}{\partial p(z \cond x) } \int_{ Z',  Y} p(z' \cond y)p(y) \log \frac{q(y \cond z')}{q(y \cond \varnothing)} \nonumber \\
%
&= \int_{ Z',  Y} p(x \cond  y) \delta_z(z') p(y) \log \frac{q(y \cond z')}{q(y \cond \varnothing)} \nonumber \\
%
&= \int_{Y} p(x \cond y)p(y) \log \frac{q(y \cond z')}{q(y \cond \varnothing)} \nonumber \\
%
&= p(x) \int_{ Y} p(y \cond x) \log \frac{q( y \cond z)}{p(y)} \frac{q(y \cond z')}{q(y \cond \varnothing)} \nonumber  \\
%
&= - p(x) \biggl( \KL{p( Y \cond x), q(Y \cond z)} \nonumber  \\
& - \KL{p( Y \cond x), p(Y)} 
 \biggr) 
\end{align*}

\begin{align*}
%%%%%%%%%
\partial_{\rv z , \rv x} &\defeq 
\frac{\partial}{\partial p(z \cond x) } \op{I}{ X;  Z} \\
&= \frac{\partial}{\partial p(z \cond x) } \int_{ Z',  X'} p(z' \cond x')p(x') \log \frac{p(z' \cond x')}{p(z')} \nonumber \\
%
&= \int_{ Z',  X'} \delta_z( z')\delta_x( x') p(x') \log \frac{p(z' \cond x')}{p(z')} \nonumber \\
&+ \int_{ Z',  X'} p(x') \frac{p(z')\delta_x(x') - p(x)}{p(z' \cond x')p(z')} \delta_z( z')
\nonumber \\
%
&=  p(x) \log \frac{p(z \cond x)}{p(z)}  
+ \int_{ X'} p(x')  \delta_x(x') \\
&- \int_{ X'} p(x' \cond z) p(x) 
\nonumber \\
%
&=  p(x) \br{\log \frac{p(z \cond  x)}{p(z)}  + 1 - 1}
\nonumber \\
%
&=  p(x) \log \frac{p(z \cond x)}{p(z)}
\end{align*}

We can now minimize the Lagrangian [eqn]:

\begin{align*} 
0 &= \frac{\partial}{\partial p(z \cond x) } \op{\mathcal{L}}{p( Z \cond  X)} \nonumber \\
%
&= \partial_{\rv z , \rv x} - \beta \partial_{\rv z \to \rv y} 
\\
%
&= p(x) \biggl( \log \frac{p(z \cond x)}{p(z)}  + \beta \KL{p( Y \cond x), q(Y \cond z)}  \\
& - \beta \KL{p( Y \cond x), q(Y \cond \varnothing)} \biggr) \\
%
\log p(z \cond x) &= \log p(z) - \beta \KL{p( Y \cond x), q(Y \cond z)} \\
&+ \beta \KL{p( Y \cond x), q(Y \cond \varnothing)}  \\
%
 p(z \cond x) &= \frac{p(z)}{C(Y,x,\beta)}\exp \pa{- \beta \KL{p( Y \cond x), q(Y \cond z)}} 
\end{align*}

With $C(Y,x,\beta) = \exp \pa{- \beta \KL{p( Y \cond x), q(Y \cond \varnothing)}}$

Let us now replace $q(\rv Y \cond \rv Z)$ and $q'(\rv Y \cond \varnothing)$ with their definitions.
Note that $q(\rv Y \cond \rv Z)$ depends itself on $p(z \cond x) $, which is why we needed to use an oracle that provides us with the optimal $q(\rv Y \cond \rv Z)$ \textit{conditioned} on the optimal $p(z \cond x)$ which we are looking for.

%We assumed that every function $q \in \mathcal{Q}$ outputs a valid distribution over $\mathcal{Z}$.
%A very similar derivation can be done in the more general case by constraining $\int_{ Z} p(z \cond  x) = 1 \ \forall x \in \mathcal{X}$, which would add $\int_{ X} \lambda(x) \br{\int_{ Z} p(z \cond  x) - 1 }$ to the Lagrangian.
%This term would not change [eqn], as it would result in adding $\lambda(x)$ in the exponent of $C(\rv Y, x, \beta)$.
\end{proof}

\blahut*


\begin{proof}
For the main parts of the proof, we refer the reader to the same theorem with vanilla information bottleneck \cite{tishby2000information}.
Here, we only prove that the theorem still holds with our changes, namely when replacing $\KL{p( Y \cond x), p(Y \cond z)}$ with $\KL{p( Y \cond x), q(Y \cond z)}$ and adding the [last self consitent eqn].

First, note that the parts of \cite{tishby2000information} proofs that depend on $\KL{p( Y \cond x), p(Y \cond z)}$ only uses the positivity of the term. 
This still holds when replacing $p(Y \cond \rv z)$ with $q(Y \cond \rv z)$.

Now, to prove convergence, we have to show that the Lagrangian [eqn] decreases at every [last self consitent eqn].

\begin{align*}
\CHF{Y}{X}^{t+1} &<  \CHF{Y}{X}^{t} \\
\op{H_\mathcal{Q}}{Y} - \CHF{Y}{X}^{t+1} &> \op{H_\mathcal{Q}}{Y} - \CHF{Y}{X}^{t} \\
\DIF{Z}{Y}^{t+1} &> \DIF{Z}{Y}^{t} \\
-\beta \DIF{Z}{Y}^{t+1} &< -\beta \DIF{Z}{Y}^{t} \\
\MI{Z}{X} -\beta \DIF{Z}{Y}^{t+1} &< \MI{Z}{X} -\beta \DIF{z}{Y}^{t} \\
\op{\mathcal{L}}{q^{t+1}(Y \cond \rv z)} &< \op{\mathcal{L}}{q^{t}(Y \cond \rv z)} 
\end{align*}

Where we have used the fact that $\MI{Z}{X}$ and $\op{H_\mathcal{Q}}{Y}$ are independent of  $q(Y \cond \rv z)$.

\end{proof}

Importantly from a practical perspective, the last self-consistent equation just requires  $q^{t+1}(Y \cond z)$ to be ``better'' than the previous one (if it can). 
It does not require to chose the best possible $q$ in the functional class $\mathcal{Q}$ which would usually be computationally infeasible.

It is also important to note that the Blahut-Arimoto algorithm was 
\begin{inlinelist}
\item Convex in the vanilla rate distortion setting; 
\item Conditionally convex (but not jointly) in the information bottleneck setting;
\item Not conditionally convex in the DIB (due to last self-consistent equation) but still convergent.
\end{inlinelist}
